# Supplementary material for: Unified Description of the Aharonov-Bohm Effect in Isotropic Multiband Electronic Systems
Source: arXiv:2302.07050 source file (2023-02-16)
Supplement: Supplementary file 1 [file AB_isotropic_theory_supplhand.tex]

\documentclass[aps,prb,superscriptaddress]{revtex4-2}

\usepackage{amsmath}
\usepackage{amssymb}
\usepackage{graphicx}
\usepackage{epsfig}
\usepackage{subcaption}
\usepackage{xcolor}
\usepackage{soul}
\usepackage{xr}

\makeatletter
\newcommand*{\addFileDependency}[1]{% argument=file name and extension
	\typeout{(#1)}% latexmk will find this if $recorder=0 (however, in that case, it will ignore #1 if it is a .aux or .pdf file etc and it exists! if it doesn't exist, it will appear in the list of dependents regardless)
	\@addtofilelist{#1}% if you want it to appear in \listfiles, not really necessary and latexmk doesn't use this
	\IfFileExists{#1}{}{\typeout{No file #1.}}% latexmk will find this message if #1 doesn't exist (yet)
}
\makeatother

\newcommand*{\myexternaldocument}[1]{%
	\externaldocument{#1}%
	\addFileDependency{#1.tex}%
	\addFileDependency{#1.aux}%
}

\myexternaldocument{AB_isotropic_theory}

\newcommand{\euler}{\mathrm{e}}
\newcommand{\iu}{\mathrm{i}}
\newcommand{\QED}{\null\nobreak\hfill\ensuremath{\blacksquare}}
\newcommand{\jav}[1]{\textcolor{red}{#1}}

\begin{document}
	
	\title{Supplemental Material: Unified Description of the Aharonov--Bohm Effect in Isotropic Multiband Electronic Systems}
	
	\author{R\'obert N\'emeth }
	
	\author{ J\'ozsef Cserti}
	%\email[Corresponding author. e-mail:]{cserti@elte.hu}
	
	\affiliation{Department of Physics of Complex Systems,
		ELTE E{\"o}tv{\"o}s Lor{\'a}nd University
		\\ H-1117 Budapest, P\'azm\'any P{\'e}ter s{\'e}t\'any 1/A, Hungary}
	
	%%%%%%%%%%%%%%%%%%%%%%%%%%
	
	\label{x_op-Q-main-shift:eq}
	
	\maketitle
	
	
	In this Supplemental Material, we present additional calculations complementing the statements of the main text. These include rigorous mathematical proofs,  detailed  derivations, and applications providing a solid footing for the paper, but they are not essential to understanding our results.
	
	
	\section{Construction of the Scattering State}
	
	In the following sections, we give rigorous mathematical proofs that conditions (i), (ii) and (iii) of the main text indeed hold for the integral representation given in Eq.~(5) of the main text. All of the proceeding calculations are novel
	results of the authors.
	
	\subsection{Condition (i): Convergence and Single-Valuedness}
	
	Although the trial solution given in Eq.~(5) of the main text might seem well-defined, in fact, there are a couple of details that need to be addressed. First of all, the plane wave solution $\boldsymbol{\Psi}_{s,\boldsymbol{k}}$ is not unique. Namely, isotropy has an effect on the \emph{momentum space eigenvectors} $\mathbf{u}_s(\boldsymbol{k})$: they transform according to the unitary maps generated by the inner angular momentum operators:
	\begin{equation}
		\hat{S}_z = \frac{\hbar}{2} \begin{pmatrix}
			D - 1 & 0 & \hdots & 0 \\
			0 & D - 3 & \hdots & 0 \\
			\vdots & \vdots & \ddots & \vdots \\
			0 & 0 & \hdots & 1 - D
		\end{pmatrix} .
		\label{eqMath1}
	\end{equation} Additionally, we can choose the phase of the eigenvector freely at every point, that is, we have a \emph{gauge freedom}. These two effects can be combined to obtain:
	\begin{equation}
		\forall \vartheta\in[0,2\pi):~~~ \mathbf{u}_s(k,\vartheta) = \euler^{\iu\chi(\vartheta)}\exp\left(-\frac{\iu}{\hbar}\vartheta\hat{S}_z\right) \mathbf{u}_s(k,0) .
		\label{eqMath2}
	\end{equation} 
	
	However, the \emph{regularity} requirement postulated in the main text reduces this freedom to a certain subset. More concretely, if the $a$th component ($1\le a \le D$) is meant to be regular, a correct gauge choice is
	\begin{equation}
		\chi(\vartheta) = \frac{(D + 1 - 2a)\vartheta}{2}  .
		\label{eqMath3}
	\end{equation} In other words, the $a$th component of the vectors $\mathbf{u}_s(k,\vartheta)$ must be independent of the polar angle $\vartheta$. The proof of regularity is not trivial even in this case, thereby it is given in detail below.
	
	\vspace{5pt}
	\noindent\textbf{\textsl{Lemma:}} The gauge choice defined in Eq.\ \eqref{eqMath3} is equivalent to the $a$th component of the momentum space eigenvectors being independent of the polar angle $\vartheta$.
	
	\vspace{5pt}
	\noindent\textbf{\textsl{Proof:}} Assume first that $a=1$. Then substituting Eqs.\ \eqref{eqMath1} and \eqref{eqMath3} into Eq.\ \eqref{eqMath2}, we can obtain the explicit form of the transformation of momentum space eigenvectors:
	\begin{equation}
		\mathbf{u}_s(k,\vartheta) = \begin{pmatrix}
			~~1~~ & ~~0~~ & \hdots & 0 \\
			~0~ & \euler^{\iu\vartheta} & \hdots & 0 \\
			\vdots & \vdots & \ddots & \vdots \\
			~0~ & ~0~ & \hdots & \euler^{\iu(D - 1)\vartheta} \\
		\end{pmatrix} \mathbf{u}_s(k,0) .
		\label{eqMath4}
	\end{equation} We can clearly see that the first component is invariant under the transformation thereby it cannot depend on $\vartheta$. If $a\neq 1$ then the above matrix is modified such that the $a$th diagonal element is unity, in that case, the $a$th component is independent of $\vartheta$. This completes the proof.\QED
	
	\vspace{5pt}
	\noindent\textbf{\textsl{Proposition:}} If the $a$th component of the momentum space eigenvectors is independent of $\vartheta$ then the $a$th component of the scattering state defined in Eq.~(5) of the main text is regular at the origin.
	
	\vspace{5pt}
	\noindent\textbf{\textsl{Proof:}} Using the assumption of the proposition, the $a$th component of the momentum space eigenvectors $\mathbf{u}_s(\boldsymbol{k})$ can be chosen as one, without the loss of generality. Therefore the $a$th component of the scattering state, based on Eq.~(5) of the main text, takes the form:
	\begin{equation}
		\Psi^{(+)}_{s,\boldsymbol{k};a}(r,\varphi) = \sum_{m = -\infty}^{\infty} \frac{\epsilon(m+\alpha)}{2\pi} \int\displaylimits^{\phantom{\Gamma}}_{\Gamma(m+\alpha,\varphi)}\mathrm{d}\xi~ \euler^{\iu kr \cos(\vartheta - \xi)} \euler^{\iu m(\xi - \vartheta) - \iu\alpha(\varphi - \xi)} ,
		\label{eqMath5a}
	\end{equation} and evaluation at the origin $r=0$ results in:
	\begin{equation}
		\Psi^{(+)}_{s,\boldsymbol{k};a}(0,\varphi) = \sum_{m = -\infty}^{\infty} \frac{\epsilon(m+\alpha)\euler^{-\iu m \vartheta-\iu\alpha\varphi}}{2\pi} \int\displaylimits^{\phantom{\Gamma}}_{\Gamma(m+\alpha,\varphi)}\mathrm{d}\xi~ \mathrm{e}^{\iu (m+\alpha)\xi} .
		\label{eqMath5}
	\end{equation} The contour integral appearing in the above expression can be easily calculated, but we ought to separate three cases. If $m+\alpha = 0$, then the integrand is unity and the contour $\Gamma_+(\varphi)$ depicted in Fig.~1 of the main text can be deformed into a $\sqcup$-shaped curve such that its segments are either parallel to the imaginary axis or running on the real axis. The contributions of the former vanish due to periodicity and the remaining part gives $2\pi$. If $m+\alpha > 0$, then the integrand is a holomorphic function approaching zero towards $\mathrm{Re}(\xi) + \iu\infty$ while the curve $\Gamma_+(\varphi)$ can be continuously shifted upwards by an arbitrary imaginary unit. Due to Cauchy's theorem \cite{Arfken}, these together imply that the value of the integral in question must be zero. A similar argument holds for $m+\alpha<0$. Altogether we can see that for $\alpha\in\mathbb{Z}$ only one term does not vanish in the series:
	\begin{equation}
		\Psi^{(+)}_{s,\boldsymbol{k};a}(0,\varphi) = \euler^{\iu\alpha(\vartheta-\varphi)} ,
		\label{eqMath6}
	\end{equation} whereas for $\alpha\notin\mathbb{Z}$ every term vanishes:
	\begin{equation}
		\Psi^{(+)}_{s,\boldsymbol{k};a}(0,\varphi) = 0 .
		\label{eqMath7}
	\end{equation} In either case, the scattering state is regular which completes the proof.\QED
	
	\vspace{5pt}
	The next non-trivial issue regarding the scattering state is whether the contour integrals and the function series appearing in its definition are convergent for all $(r,\varphi)$. The proof can be given for a general multiband electronic system, this is presented below separately for $\alpha\in\mathbb{Z}$ and $\alpha\notin\mathbb{Z}$. The former case is simpler and thereby given first.
	
	\vspace{5pt}
	\noindent\textbf{\textsl{Proposition:}} The scattering states defined in Eq.~(5) of the main text are convergent for $\alpha\in\mathbb{Z}$.
	
	\vspace{5pt}
	\noindent\textbf{\textsl{Proof:}} With the constraint of $\alpha\in\mathbb{Z}$, the integrand in the trial solution becomes periodic along the real axis with a period of $2\pi$. Let us deform the contours $\Gamma_\pm(\varphi)$ into $\sqcup$-shaped and $\sqcap$-shaped curves such that its segments are either parallel to the imaginary axis or running on the real axis. The contributions of the former vanish due to periodicity and the following expression remains:
	\begin{equation}
		\boldsymbol{\Psi}^{(+)}_{s,\boldsymbol{k}}(r,\varphi) = \sum_{m = -\infty}^{\infty} \frac{\mathrm{e}^{-\iu m\vartheta}}{2\pi}\int_{-\pi}^\pi \mathrm{d}\xi~ \boldsymbol{\Psi}_{s,\boldsymbol{K}}(r,\varphi) \mathrm{e}^{\iu m\xi} ,
		\label{eqMath29}
	\end{equation} where $\boldsymbol{K} = k[\cos\xi,\sin\xi]$ as introduced in the main text. The right-hand side is manifestly the Fourier expansion of the plane wave solution with respect to the variable $-\xi$, that is, for the $\alpha = 0$ case:
	\begin{equation}
		\boldsymbol{\Psi}^{(+)}_{s,\boldsymbol{k}}(r,\varphi) = \boldsymbol{\Psi}_{s,\boldsymbol{k}}(r,\varphi) .
		\label{eqMath30}
	\end{equation} The more general case of $\alpha\in\mathbb{Z}$ can be retraced to the above result by performing the variable change $m \to m + \alpha$. In this case, the scattering state is a plane wave multiplied by the phase factor given in Eq.~\eqref{eqMath6}. \QED
	
	\vspace{5pt}
	Next, we can turn to the case of $\alpha\notin\mathbb{Z}$. To this end, recall the \emph{partial waves} $\mathbf{U}_{s,k,m}$ introduced in Eq.~(12) of the main text by an implicit definition:
	\begin{equation}
		\boldsymbol{\Psi}^{(+)}_{s,\boldsymbol{k}}(r,\varphi) = \sum_{m=-\infty}^\infty \hspace{-5pt}  {\left(-\iu \right)}^{|m+\alpha|} \euler^{\iu m(\pi - \vartheta)} \mathbf{U}_{s,k,m}(r,\varphi) .
		\label{eqMath8}
	\end{equation}
	
	\vspace{5pt}
	\noindent\textbf{\textsl{Lemma:}} The partial waves defined in Eq.\ \eqref{eqMath8} are convergent for $\alpha\notin\mathbb{Z}$.
	
	\vspace{5pt}
	\noindent\textbf{\textsl{Proof:}} By definition, the partial waves can be written as:
	\begin{equation}
		\mathbf{U}_{s,k,m}(r,\varphi) = \frac{\epsilon(m+\alpha)\iu^{|m+\alpha|}\euler^{-\iu m\pi}}{2\pi}\int\displaylimits^{\phantom{\Gamma}}_{\Gamma(m+\alpha,\varphi)}\mathrm{d}\xi~ \boldsymbol{\Psi}_{s,\boldsymbol{K}}(r,\varphi) \mathrm{e}^{\iu (m+\alpha) \xi - \iu\alpha\varphi} .
		\label{eqMath9}
	\end{equation} Since the integrand appearing in the above expression is a holomorphic function for each component, it suffices to prove that the integral is finite. To this end, consider first the case with $m+\alpha\ge 0$ and $v_{s,k}(\boldsymbol{k})>0$ when the contour $\Gamma(m+\alpha,\varphi)$ becomes the $\Gamma_+(\varphi)$ depicted in Fig.~1 of the main text. The integration contour can then be deformed to a $\sqcup$-shaped curve again separating Eq.\ \eqref{eqMath9} into three integrals $I_{s,k,m}^{(1)}(r,\varphi)$, $I_{s,k,m}^{(2)}(r,\varphi)$ and $I_{s,k,m}^{(3)}(r,\varphi)$ as
	\begin{subequations}
		\begin{align}
			I_{s,k,m}^{(1)}(r,\varphi) &= \frac{(-\iu)^{m-\alpha}\euler^{-\iu\alpha\varphi}}{2\pi}\int\displaylimits_{-5\pi/2 + \varphi + \iu\infty}^{-5\pi/2 + \varphi + \iu\varepsilon} \mathrm{d}\xi~ \boldsymbol{\Psi}_{s,\boldsymbol{K}}(r,\varphi) \mathrm{e}^{\iu (m+\alpha)\xi} , 
			\label{eqMath10a} \\
			I_{s,k,m}^{(2)}(r,\varphi) &= \frac{(-\iu)^{m-\alpha}\euler^{-\iu\alpha\varphi}}{2\pi}\int\displaylimits_{-5\pi/2 + \varphi + \iu\varepsilon}^{-\pi/2 + \varphi + \iu\varepsilon} \mathrm{d}\xi~ \boldsymbol{\Psi}_{s,\boldsymbol{K}}(r,\varphi) \mathrm{e}^{\iu (m+\alpha)\xi} , 
			\label{eqMath10b} \\
			I_{s,k,m}^{(3)}(r,\varphi) &= \frac{(-\iu)^{m-\alpha}\euler^{-\iu\alpha\varphi}}{2\pi}\int\displaylimits_{-\pi/2 + \varphi + \iu\varepsilon}^{-\pi/2 + \varphi + \iu\infty} \mathrm{d}\xi~ \boldsymbol{\Psi}_{s,\boldsymbol{K}}(r,\varphi) \mathrm{e}^{\iu (m+\alpha)\xi} . 
			\label{eqMath10c}
		\end{align}
	\end{subequations} Here $\varepsilon\in\mathbb{R}^+$ is an arbitrary positive real number. The second integral is manifestly finite as its domain is a compact set, the first and the third need further investigation. Consider the plane wave term in the integrand evaluated on one of these segments. With the gauge choice given in Eq.\ \eqref{eqMath3}, the $b$th component is (up to a constant multiplier) given as:
	\begin{equation}
		\Psi_{s,\boldsymbol{K};b}(r,\varphi) = \euler^{\iu kr \cos(\varphi - \xi) + \iu (b-a)\xi} = (-\iu)^{b-a} \euler^{\iu (b-a) \varphi} \euler^{- kr \sinh\left[\mathrm{Im}(\xi)\right] + (a-b) \mathrm{Im}(\xi)}  .
		\label{eqMath11}
	\end{equation} For any $kr\in\mathbb{R}^+$ and $a,b\in\mathbb{Z}$, the function $(a-b)\mathrm{Im}(\xi)$ is linearly increasing whereas the function $kr\sinh\left[\mathrm{Im}(\xi)\right]$ is exponentially increasing as $\mathrm{Im}(\xi)\to\infty$. Therefore above a certain limiting point $\mathrm{Im}(\xi) = \delta$, the real term $\euler^{- kr \sinh\left[\mathrm{Im}(\xi)\right] + (a-b) \mathrm{Im}(\xi)}$ becomes smaller than one. Choosing $\varepsilon > \delta$, the $b$th component of the integrals in Eqs.\ \eqref{eqMath10a} and \eqref{eqMath10c} have the following upper bound:
	\begin{subequations}
		\begin{align}
			\left|I_{s,k,m;b}^{(1)}(r,\varphi)\right| &\le \frac{1}{2\pi}\int\displaylimits_{\varepsilon}^{\infty} \mathrm{d}\hspace{1pt}\mathrm{Im}(\xi)~  \mathrm{e}^{- (m+\alpha)\mathrm{Im}(\xi)} = \frac{\mathrm{e}^{-(m+\alpha)\varepsilon}}{2(m + \alpha)\pi} , 
			\label{eqMath12a} \\
			\left|I_{s,k,m;b}^{(3)}(r,\varphi)\right| &\le \frac{1}{2\pi}\int\displaylimits_{\varepsilon}^{\infty} \mathrm{d}\hspace{1pt}\mathrm{Im}(\xi)~  \mathrm{e}^{- (m+\alpha)\mathrm{Im}(\xi)} = \frac{\mathrm{e}^{-(m+\alpha)\varepsilon}}{2(m + \alpha)\pi} .
			\label{eqMath12b}
		\end{align}
	\end{subequations} This is clearly finite for any $m\in\mathbb{Z}$ whenever $\alpha\notin\mathbb{Z}$. In summary, all the three terms in Eqs.\ \eqref{eqMath10a}, \eqref{eqMath10b} and \eqref{eqMath10c}, and thereby the complete integral in Eq.\ \eqref{eqMath9} are convergent. The generalization of the previous calculations to the cases with $m+\alpha<0$ or $v_{s,k}(\boldsymbol{k})<0$ is straightforward. This completes the proof.\QED
	
	\vspace{5pt}
	\noindent\textbf{\textsl{Proposition:}} The scattering states defined in Eq.~(5) of the main text are convergent for $\alpha\notin\mathbb{Z}$.
	
	\vspace{5pt}
	\noindent\textbf{\textsl{Proof:}} A well-known theorem of complex analysis \cite{Arfken} states that a series of contour integrals
	\begin{equation}
		I = \sum_{m=0}^\infty \int\displaylimits_{\Gamma} \mathrm{d}z~f_m(z)
		\label{eqMath13}
	\end{equation} exists and summation is interchangeable with integration, that is:  
	\begin{equation}
		I = \int\displaylimits_{\Gamma} \mathrm{d}z~\sum_{m=0}^\infty f_m(z),
		\label{eqMath14}
	\end{equation} if the integrand of the latter expression is uniformly convergent and its limit is integrable. Consequently, the proof of our proposition requires the verification of the aforementioned properties. To this end, separate the summation over $m$ into two parts corresponding to $m+\alpha \ge 0$ and $m+\alpha < 0$. The resulting function series contain only integrals along the curves $\Gamma_+(\varphi)$ and $\Gamma_-(\varphi)$, respectively. These contours are such that either $\mathrm{Im}\xi > 0$ or $\mathrm{Im}\xi < 0$ is satisfied along them. Then the following function series appear in the integrands:
	\begin{subequations}
		\begin{align}
			&\mathrm{Im}(\xi) > 0:~~~\sum_{m = -\lfloor\alpha\rfloor}^\infty \mathrm{e}^{\iu m(\xi - \vartheta)}, \label{eqMath15a} \\
			&\mathrm{Im}(\xi) < 0:~~~\sum_{m = -\infty}^{-\lfloor\alpha\rfloor - 1} \mathrm{e}^{\iu m(\xi - \vartheta)}. \label{eqMath15b}
		\end{align}
	\end{subequations} These are simple geometric series that are uniformly convergent owing to the relation $\mathrm{Im}(\vartheta) = 0$. Substituting the well-known formula of the limit leads to the alternative form of the scattering states:
	\begin{equation}
		\begin{aligned}
			\boldsymbol{\Psi}^{(+)}_{s,\boldsymbol{k}}(r,\varphi) &= \frac{\iu}{4\pi}\int\displaylimits_{\Gamma_+(\varphi)\cup\Gamma_-(\varphi)}\mathrm{d}\xi~ \boldsymbol{\Psi}_{s,\boldsymbol{K}}(r,\varphi) \frac{\mathrm{e}^{\iu\alpha(\xi - \varphi)} \mathrm{e}^{\iu\left(\lfloor\alpha\rfloor + \frac12\right)(\vartheta - \xi)}}{\sin\left(\frac{\xi - \vartheta}{2}\right)} ,
		\end{aligned}
		\label{eqMath16}
	\end{equation} where $\lfloor\bullet\rfloor$ denotes the floor function. Note that the integral is taken along the concatenation of contours $\Gamma_+(\varphi)$ and $\Gamma_-(\varphi)$, which can also be regarded as the sum of two separate integrals along the aforementioned contours. As a final step, we need to show that these integrals are finite. Consider first the integral over $\Gamma_+(\varphi)$ and assume that $v_{s,k}(\boldsymbol{k})>0$. As before, the integration contour can then be deformed to a $\sqcup$-shaped curve separating Eq.\ \eqref{eqMath16} into three integrals $I_{s,\boldsymbol{k}}^{(1)}(r,\varphi)$, $I_{s,\boldsymbol{k}}^{(2)}(r,\varphi)$ and $I_{s,\boldsymbol{k}}^{(3)}(r,\varphi)$:
	\begin{subequations}
		\begin{align}
			I_{s,\boldsymbol{k}}^{(1)}(r,\varphi) &= \frac{\iu \euler^{-\iu\alpha\varphi} \euler^{\iu\left(\lfloor\alpha\rfloor + \frac12\right)\vartheta}}{4\pi}\int\displaylimits_{-5\pi/2 + \varphi + \iu\infty}^{-5\pi/2 + \varphi + \iu\varepsilon} \mathrm{d}\xi~ \boldsymbol{\Psi}_{s,\boldsymbol{K}}(r,\varphi) \frac{\euler^{\iu\left(\{\alpha\} - \frac12\right)\xi}}{\sin\left(\frac{\xi - \vartheta}{2}\right)} , 
			\label{eqMath17a} \\
			I_{s,\boldsymbol{k}}^{(2)}(r,\varphi) &= \frac{\iu \euler^{-\iu\alpha\varphi} \euler^{\iu\left(\lfloor\alpha\rfloor + \frac12\right)\vartheta}}{4\pi}\int\displaylimits_{-5\pi/2 + \varphi + \iu\varepsilon}^{-\pi/2 + \varphi + \iu\varepsilon} \mathrm{d}\xi~ \boldsymbol{\Psi}_{s,\boldsymbol{K}}(r,\varphi) \frac{\euler^{\iu\left(\{\alpha\} - \frac12\right)\xi}}{\sin\left(\frac{\xi - \vartheta}{2}\right)}, 
			\label{eqMath17b} \\
			I_{s,\boldsymbol{k}}^{(3)}(r,\varphi) &= \frac{\iu \euler^{-\iu\alpha\varphi} \euler^{\iu\left(\lfloor\alpha\rfloor + \frac12\right)\vartheta}}{4\pi}\int\displaylimits_{-\pi/2 + \varphi + \iu\varepsilon}^{-\pi/2 + \varphi + \iu\infty} \mathrm{d}\xi~ \boldsymbol{\Psi}_{s,\boldsymbol{K}}(r,\varphi) \frac{\euler^{\iu\left(\{\alpha\} - \frac12\right)\xi}}{\sin\left(\frac{\xi - \vartheta}{2}\right)}. 
			\label{eqMath17c}
		\end{align}
	\end{subequations} Here $\varepsilon\in\mathbb{R}^+$ is an arbitrary positive real number. The second integral is manifestly finite as its domain is a compact set, the first and the third need further investigation. Choosing $\varepsilon>\log(2)/2$, consider the following estimation on one of these segments:
	\begin{equation}
		\mathrm{Im}(\xi)\ge\varepsilon:~~~\left|\sin\left(\frac{\xi - \vartheta}{2}\right)\right| \ge \sinh\left[\frac{\mathrm{Im}(\xi)}{2}\right] \ge \frac14 \exp\left[\frac{\mathrm{Im}(\xi)}{2}\right] .
		\label{eqMath18}
	\end{equation} Using this and the expression for the plane wave term expounded in Eq.\ \eqref{eqMath11}, an upper bound for the $b$th component of the integrals in Eqs.\ \eqref{eqMath17a} and \eqref{eqMath17c}, while choosing $\varepsilon>\max[\delta,\log(2)/2]$, reads:
	\begin{subequations}
		\begin{align}
			\left|I_{s,\boldsymbol{k};b}^{(1)}(r,\varphi)\right| &\le \frac{1}{\pi}\int\displaylimits_{\varepsilon}^{\infty} \mathrm{d}\hspace{1pt}\mathrm{Im}(\xi)~ \euler^{-\{\alpha\}\mathrm{Im}(\xi)} = \frac{\euler^{-\{\alpha\}\varepsilon}}{\{\alpha\}\pi} , 
			\label{eqMath19a} \\
			\left|I_{s,\boldsymbol{k};b}^{(3)}(r,\varphi)\right| &\le \frac{1}{\pi}\int\displaylimits_{\varepsilon}^{\infty} \mathrm{d}\hspace{1pt}\mathrm{Im}(\xi)~ \euler^{-\{\alpha\}\mathrm{Im}(\xi)} = \frac{\euler^{-\{\alpha\}\varepsilon}}{\{\alpha\}\pi} . \label{eqMath19b}
		\end{align}
	\end{subequations} This is clearly finite whenever $\alpha\notin\mathbb{Z}$. In summary, all the three terms in Eqs.\ \eqref{eqMath17a}, \eqref{eqMath17b} and \eqref{eqMath17c}, and thereby the complete integral in Eq.\ \eqref{eqMath16} are convergent. The generalization of the previous calculations to the contour $\Gamma_-(\varphi)$ or the case of $v_{s,k}(\boldsymbol{k})<0$ is straightforward. This completes the proof.\QED 
	
	\vspace{5pt}
	The only remaining question is that of single-valuedness which is essentially non-trivial since the trial solution was defined in terms of coordinates. To prove it, one needs to check whether the substitutions of any $\varphi\in\mathbb{R}$ and $\varphi + 2\pi$ return the same value. Using the definitions of the contours $\Gamma_\pm(\varphi)$ given in the main text, and performing a change of variables $\xi \to \xi - 2\pi$, the following results are simply obtained:
	\begin{equation}
		\boldsymbol{\Psi}^{(+)}_{s,\boldsymbol{k}}(r,\varphi + 2\pi) = \boldsymbol{\Psi}^{(+)}_{s,\boldsymbol{k}}(r,\varphi) .
		\label{eqMath20}
	\end{equation} With this problem resolved, the trial solution is now rigorously defined.
	
	
	\subsection{Condition (ii): Eigenvector Property}
	
	Having a well-defined trial solution, one needs to show that it satisfies the time-independent Schrödinger equation, that is, whether it is an eigenvector of the Hamiltonian operator. To this end, we first have to prove that the Hamiltonian can be exchanged with the infinite sum and contour integral appearing in the trial solution. This is shown in the following for $\alpha\notin\mathbb{Z}$, whereas the case of $\alpha\in\mathbb{Z}$ is trivial based on the previous subsection. 
	
	\vspace{5pt}
	\noindent\textbf{\textsl{Proposition:}} The Hamiltonian operator defined in Eq.~(4) of the main text can be interchanged with the summation and integration appearing in the scattering states of Eq.~(5) of the main text for $\alpha\notin\mathbb{Z}$.
	
	\vspace{5pt}
	\noindent\textbf{\textsl{Proof:}} The Leibniz integral rule applicable for complex integrals \cite{Arfken} states that the derivative of a contour integral depending on some real parameter $x\in\mathbb{R}$
	\begin{equation}
		I(x) = \int\displaylimits_{a(x)}^{b(x)} \mathrm{d}z~f(z,x)
		\label{eqMath21}
	\end{equation} can be expressed as
	\begin{equation}
		I'(x) = f(b(x),x)~b'(x) - f(a(x),x)~a'(x) + \int\displaylimits_{a(x)}^{b(x)} \mathrm{d}z~\partial_x f(z,x)
		\label{eqMath22}
	\end{equation} provided that $f$ is holomorphic in a neighborhood of the integration curve and the absolute value of $\partial_x f(z,x)$ is bounded from above independently of $x$. In our case, the Hamiltonian is a polynomial of operators $\hat{\Pi}_x$ and $\hat{\Pi}_y$, or equivalently, of operators $\hat{\Pi}_\pm = \hat{\Pi}_x \pm \iu\hat{\Pi}_y$ due to Eq.~(4) of the main text. Therefore, it suffices to prove that the operator $\hat{\Pi}_+^i \hat{\Pi}_-^j$ is interchangeable with the integration in Eq.~(5) of the main text. Following a similar approach as before, consider the case of the contour $\Gamma_+(\varphi)$ and $v_{s,k}(\boldsymbol{k}) > 0$ in Eq.~\eqref{eqMath16}, and perform the following separation:
	\begin{subequations}
		\begin{align}
			I_{s,\boldsymbol{k}}^{(4)}(r,\varphi) &= \frac{\iu \euler^{\iu\left(\lfloor\alpha\rfloor + \frac12\right)\vartheta}}{4\pi}\int\displaylimits_{-5\pi/2 + \varphi + \iu\infty}^{-5\pi/2 + \varphi + \iu\varepsilon} \mathrm{d}\xi~ \hat{\Pi}_+^i \hat{\Pi}_-^j \boldsymbol{\Psi}_{s,\boldsymbol{K}}(r,\varphi) \euler^{-\iu\alpha\varphi} \frac{\euler^{\iu\left(\{\alpha\} - \frac12\right)\xi}}{\sin\left(\frac{\xi - \vartheta}{2}\right)} , 
			\label{eqMath23a} \\
			I_{s,\boldsymbol{k}}^{(5)}(r,\varphi) &= \frac{\iu \euler^{\iu\left(\lfloor\alpha\rfloor + \frac12\right)\vartheta}}{4\pi}\int\displaylimits_{-5\pi/2 + \varphi + \iu\varepsilon}^{-\pi/2 + \varphi + \iu\varepsilon} \mathrm{d}\xi~ \hat{\Pi}_+^i \hat{\Pi}_-^j \boldsymbol{\Psi}_{s,\boldsymbol{K}}(r,\varphi) \euler^{-\iu\alpha\varphi} \frac{\euler^{\iu\left(\{\alpha\} - \frac12\right)\xi}}{\sin\left(\frac{\xi - \vartheta}{2}\right)}, 
			\label{eqMath23b} \\
			I_{s,\boldsymbol{k}}^{(6)}(r,\varphi) &= \frac{\iu \euler^{\iu\left(\lfloor\alpha\rfloor + \frac12\right)\vartheta}}{4\pi}\int\displaylimits_{-\pi/2 + \varphi + \iu\varepsilon}^{-\pi/2 + \varphi + \iu\infty} \mathrm{d}\xi~ \hat{\Pi}_+^i \hat{\Pi}_-^j \boldsymbol{\Psi}_{s,\boldsymbol{K}}(r,\varphi) \euler^{-\iu\alpha\varphi} \frac{\euler^{\iu\left(\{\alpha\} - \frac12\right)\xi}}{\sin\left(\frac{\xi - \vartheta}{2}\right)}. 
			\label{eqMath23c}
		\end{align}
	\end{subequations} Here $\varepsilon\in\mathbb{R}^+$ is an arbitrary positive real number. The second integral is manifestly finite as its domain is a compact set, the first and the third need further investigation. Consider the action of $\hat{\Pi}_\pm$ operators on the plane wave term in the integrand evaluated on one of these segments. With the gauge choice given in Eq.\ \eqref{eqMath3}, the $b$th component is given as:
	\begin{equation}
		\hat{\Pi}_+^i \hat{\Pi}_-^j \big[\Psi_{s,\boldsymbol{K};b}(r,\varphi)\euler^{-\iu\alpha\varphi}\big] = (\hbar k)^{i+j}(-\iu)^{b-a+i-j} \euler^{\iu (a-b+i-j) \varphi} \euler^{- kr \sinh\left[\mathrm{Im}(\xi)\right] + (b-a+i-j) \mathrm{Im}(\xi)}  .
		\label{eqMath24}
	\end{equation} For any $kr\in\mathbb{R}^+$ and $a,b,i,j\in\mathbb{Z}$, the function $(b-a+i-j)\mathrm{Im}(\xi)$ is linearly increasing whereas the function $kr\sinh\left[\mathrm{Im}(\xi)\right]$ is exponentially increasing as $\mathrm{Im}(\xi)\to\infty$. Therefore above a certain limiting point $\mathrm{Im}(\xi) = \delta$, the real term $\euler^{- kr \sinh\left[\mathrm{Im}(\xi)\right] + (b-a+i-j) \mathrm{Im}(\xi)}$ becomes smaller than one. Choosing $\varepsilon > \delta$, the $b$th component of Eqs.\ \eqref{eqMath23a} and \eqref{eqMath23c} can be estimated:
	\begin{subequations}
		\begin{align}
			\left|I_{s,\boldsymbol{k}}^{(4)}(r,\varphi)\right| &\le \frac{(\hbar k)^{i+j}}{2\pi}\int\displaylimits_{\varepsilon}^{\infty} \mathrm{d}\hspace{1pt}\mathrm{Im}(\xi)~ \euler^{-\{\alpha\}\mathrm{Im}(\xi)} = \frac{(\hbar k)^{i+j}\euler^{-\{\alpha\}\varepsilon}}{2\pi\{\alpha\}} , 
			\label{eqMath25a} \\
			\left|I_{s,\boldsymbol{k}}^{(6)}(r,\varphi)\right| &\le \frac{(\hbar k)^{i+j}}{2\pi}\int\displaylimits_{\varepsilon}^{\infty} \mathrm{d}\hspace{1pt}\mathrm{Im}(\xi)~ \euler^{-\{\alpha\}\mathrm{Im}(\xi)} = \frac{(\hbar k)^{i+j}\euler^{-\{\alpha\}\varepsilon}}{2\pi\{\alpha\}} . \label{eqMath25b}
		\end{align}
	\end{subequations} This is clearly finite whenever $\alpha\notin\mathbb{Z}$. In summary, all the three terms in Eqs.\ \eqref{eqMath23a}, \eqref{eqMath23b}, and \eqref{eqMath23c} are convergent. Due to the Leibniz integral rule -- noting that all boundary terms vanish as the integrand is rapidly decaying, this implies the interchangeability of the differential operator and integration. The generalization of the previous calculations to the contour $\Gamma_-(\varphi)$ or the case of $v_{s,k}(\boldsymbol{k})<0$ is straightforward. This completes the proof.\QED
	
	\vspace{5pt}
	Based on the proposition above, we can continue the calculation:
	\begin{equation}
		\Big[\hat{H}\boldsymbol{\Psi}^{(+)}_{s,\boldsymbol{k}}\Big](r,\varphi) = \sum_{m = -\infty}^{\infty} \frac{\epsilon(m+\alpha)}{2\pi}\int\displaylimits_{\Gamma(m+\alpha,\varphi)}\mathrm{d}\xi~ \hat{H} \Big[\boldsymbol{\Psi}_{s,\boldsymbol{K}}(r,\varphi) \mathrm{e}^{\iu m(\xi - \vartheta) - \iu\alpha(\varphi - \xi)}\Big] .
		\label{eqMath26}
	\end{equation} Next, exploiting Eqs.~\eqref{eqMath11} and \eqref{eqMath24}, the following important identity is obtained:
	\begin{equation}
		\hat{\Pi}_+^i \hat{\Pi}_-^j \big[\Psi_{s,\boldsymbol{K}}(r,\varphi)\euler^{-\iu\alpha\varphi}\big] = \hat{p}_+^i \hat{p}_-^j \big[\Psi_{s,\boldsymbol{K}}(r,\varphi)\big]\euler^{-\iu\alpha\varphi},
		\label{eqMath27a}
	\end{equation} which in fact holds for more general wave functions as well. Together with the isotropy of the dispersion relation, this leads to:
	\begin{equation}
		\hat{H} \Big[ \boldsymbol{\Psi}_{s,\boldsymbol{K}}(r,\varphi) \mathrm{e}^{\iu m(\xi - \vartheta) - \iu\alpha(\varphi - \xi)} \Big] = E_s(k) \boldsymbol{\Psi}_{s,\boldsymbol{K}}(r,\varphi) \mathrm{e}^{\iu m(\xi - \vartheta) - \iu\alpha(\varphi - \xi)} .
		\label{eqMath27}
	\end{equation} The comparison of Eqs.\ \eqref{eqMath26} and \eqref{eqMath27} results in the quick verification of the eigenvector property:
	\begin{equation}
		\hat{H}\boldsymbol{\Psi}^{(+)}_{s,\boldsymbol{k}} = E_s(k) \boldsymbol{\Psi}^{(+)}_{s,\boldsymbol{k}} .
		\label{eqMath28}
	\end{equation} Note that the essence of the above derivation was the presence of the $\euler^{-i\alpha\varphi}$ multiplier in the integrand. This procedure has historical precursors: in earlier attempts, physicists tried solving magnetic problems by multiplying plane wave solutions by such phase factors, this is called \textit{Dirac's prescription}. However, these solutions were ill-defined when $\alpha\notin\mathbb{Z}$ as they returned different values for $\varphi = 0$ and $\varphi = 2\pi$. In our case, the multiplication is performed inside the integrand and there is an additional $\varphi$-dependence in the integration contours $\Gamma_\pm(\varphi)$ ensuring the single-valuedness as seen in the \textsl{Condition (i): Convergence and Single-Valuedness} subsection. Consequently, the general method proposed here could be regarded as an improved version of Dirac's prescription.
	
	\subsection{Condition (iii): Asymptotic Form}
	
	The examination of the trial solution is nearly finished, the only remaining task is the calculation of the asymptotic form in the $r\to\infty$ limit. To this end, we need to apply the \textit{method of steepest descent} well-known from complex analysis \cite{Arfken} to the trial solution expressed in Eq.\ \eqref{eqMath16}. The illustrative picture behind this method is that the integral in question is dominated by the exponential factor $\euler^{\iu kr\cos(\varphi - \xi)}$ appearing in the integrand which is a rapidly oscillating function. Therefore considerable contribution is only expected around \textit{saddle points} where the derivative of the exponent vanishes and its imaginary part is zero. The asymptotic form can be obtained by deforming the contour such that it touches these saddle points and the imaginary part of the exponent is constant all along. 
	
	Consequently, we first need to find the saddle points. These appear where the derivative of $\cos(\varphi - \xi)$ with respect to $\xi$ is zero, that is, at
	\begin{equation}
		\xi_n = \varphi - n\pi,~~~n\in\mathbb{Z}.
		\label{eqMath31}
	\end{equation} Around the saddle points, the cosine function can be expanded in a Taylor series:
	\begin{equation}
		\cos(\varphi - \xi) = (-1)^n - \frac{(-1)^{n}}{2} (\xi - \xi_n)^2 + \mathcal{O}\left[(\xi - \xi_n)^4\right] .
		\label{eqMath32}
	\end{equation} This expression shows that the direction in which the real part is asymptotically constant around $\xi = \xi_n$ is that of $\euler^{\iu\pi/4}$ or $\euler^{3\iu\pi/4}$ depending on whether $n$ is odd or even, respectively. Based on this, the correct deformation of the contours $\Gamma_\pm(\varphi)$ are shown in Fig.\ \ref{figMath1}. Note that the contours cross only two of the saddle points since they must avoid regions where the imaginary part of $\cos(\varphi - \xi)$ is negative, as in these regions the integrand would be infinitely large. 
	
	\begin{figure}[hbt]
		\centering
		\includegraphics[scale=0.833]{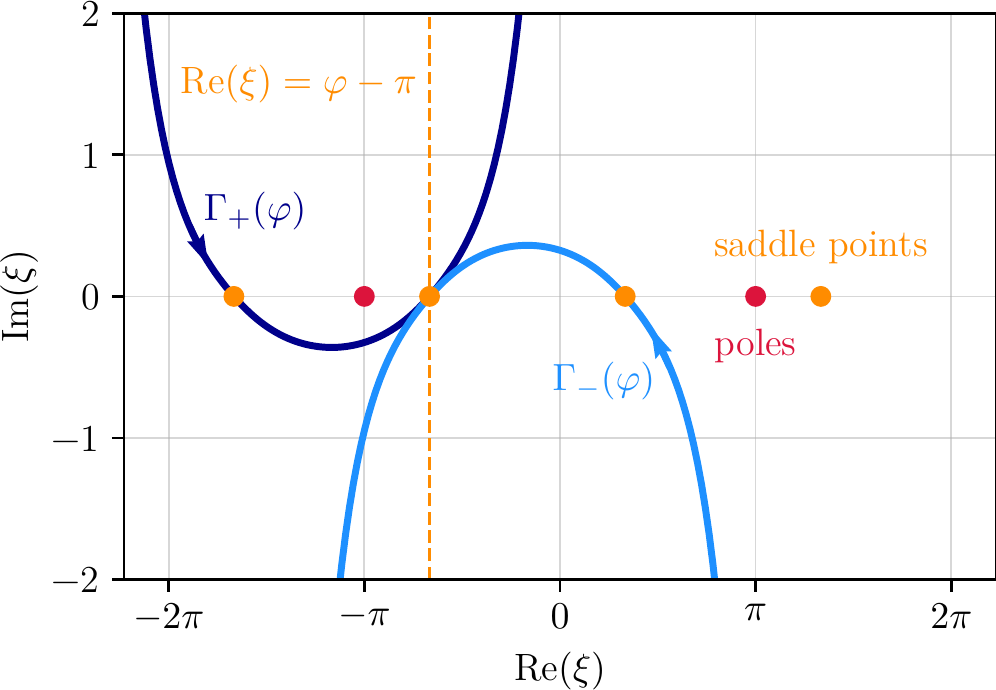}
		\hspace{10pt}
		\includegraphics[scale=0.833]{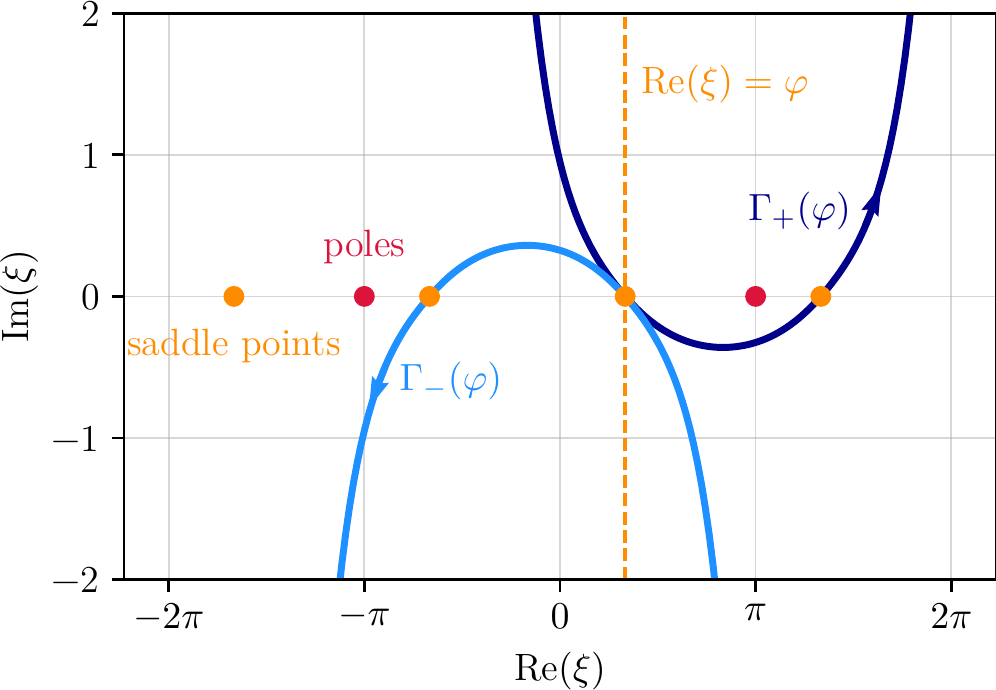}
		%\captionsetup{justification=justified,labelfont=bf,font=small,width=400pt}
		\caption{Deformation of the contours $\Gamma_\pm(\varphi)$ during the method of steepest descent for the case of $\vartheta = \pi$, $\varphi = \pi/3$, and  $v_{s,k}(\boldsymbol{k}) > 0$ (left panel) or  $v_{s,k}(\boldsymbol{k}) < 0$ (right panel). Saddle points and poles of the integrand are denoted by orange and red dots. Orange dashed lines mark the loci of $\mathrm{Re}(\xi)=\varphi - \pi$ (left panel) and $\mathrm{Re}(\xi)=\varphi$ (right panel).}
		\label{figMath1}
	\end{figure}
	
	After this preparation, the contribution of saddle points can finally be calculated. Since there are two contours, a term appears for both and they have to be summed up. The curves $\Gamma_\pm(\varphi)$ defined in Fig.~1 of the main text depend strongly on the sign of the radial group velocity, thereby the two cases ought to be separated.
	\begin{itemize}
		\item If $v_{s,k}(\boldsymbol{k})>0$ then the saddle point $\xi_{1} = \varphi - \pi$ is touched by both $\Gamma_+(\varphi)$ and $\Gamma_-(\varphi)$ in opposite directions, whereas the equivalent saddle points $\xi_{0} = \varphi$ and $\xi_{2} = \varphi - 2\pi$ are only touched by either $\Gamma_+(\varphi)$ or $\Gamma_-(\varphi)$. The prefactor appearing in the former case vanishes:
		\begin{equation}
			\frac{\iu\mathrm{e}^{\iu\alpha(\xi_1 - \varphi)} \mathrm{e}^{\iu\left(\lfloor\alpha\rfloor + \frac12\right)(\vartheta - \xi_1)}}{2\sin\left(\frac{\xi_1 - \vartheta}{2}\right)} - \frac{\iu\mathrm{e}^{\iu\alpha(\xi_1 - \varphi)} \mathrm{e}^{\iu\left(\lfloor\alpha\rfloor + \frac12\right)(\vartheta - \xi_1)}}{2\sin\left(\frac{\xi_1 - \vartheta}{2}\right)} = 0 ,
			\label{eqMath33}
		\end{equation} whereas in the latter case it does not:
		\begin{equation}
			\frac{\iu\mathrm{e}^{\iu\alpha(\xi_0 - \varphi)} \mathrm{e}^{\iu\left(\lfloor\alpha\rfloor + \frac12\right)(\vartheta - \xi_0)}}{2\sin\left(\frac{\xi_0 - \vartheta}{2}\right)} - \frac{\iu\mathrm{e}^{\iu\alpha(\xi_2 - \varphi)} \mathrm{e}^{\iu\left(\lfloor\alpha\rfloor + \frac12\right)(\vartheta - \xi_2)}}{2\sin\left(\frac{\xi_2 - \vartheta}{2}\right)} = \frac{\sin(\alpha\pi)}{\sin\left(\frac{\varphi - \vartheta}{2}\right)}\mathrm{e}^{-\iu\alpha\pi} \mathrm{e}^{\iu\left(\lfloor\alpha\rfloor + \frac12\right)(\vartheta - \varphi)} .
			\label{eqMath34}
		\end{equation} Using this, the complete contribution gives us the outgoing wave:
		\begin{equation}
			\boldsymbol{\Psi}_{s,\boldsymbol{k}}^\mathrm{out}(r,\varphi) = \frac{F(\varphi-\vartheta)}{\sqrt{r}} \euler^{\iu k r} \mathbf{u}_s(k,\varphi) ,
			\label{eqMath35}
		\end{equation} where the \emph{scattering function} $F$ takes the following form:
		\begin{equation}
			F(\varphi - \vartheta) = \frac{\sin(\alpha\pi)\euler^{-\iu\alpha\pi} \euler^{\iu\left(\lfloor\alpha\rfloor + \frac12\right)(\vartheta - \varphi)}}{\sqrt{2\pi\iu k} \sin\left(\frac{\varphi - \vartheta}{2}\right)} .
			\label{eqMath36}
		\end{equation}
		
		\item If $v_{s,k}(\boldsymbol{k})<0$ then the saddle point $\xi_{0} = \varphi$ is touched by both $\Gamma_+(\varphi)$ and $\Gamma_-(\varphi)$ in opposite directions, whereas the equivalent saddle points $\xi_{1} = \varphi - \pi$ and $\xi_{-1} = \varphi + \pi$ are only touched by either $\Gamma_+(\varphi)$ or $\Gamma_-(\varphi)$. The prefactor appearing in the former case vanishes:
		\begin{equation}
			\frac{\iu\mathrm{e}^{\iu\alpha(\xi_0 - \varphi)} \mathrm{e}^{\iu\left(\lfloor\alpha\rfloor + \frac12\right)(\vartheta - \xi_0)}}{2\sin\left(\frac{\xi_0 - \vartheta}{2}\right)} - \frac{\iu\mathrm{e}^{\iu\alpha(\xi_0 - \varphi)} \mathrm{e}^{\iu\left(\lfloor\alpha\rfloor + \frac12\right)(\vartheta - \xi_0)}}{2\sin\left(\frac{\xi_0 - \vartheta}{2}\right)} = 0 ,
			\label{eqMath37}
		\end{equation} whereas in the latter case it does not:
		\begin{equation}
			\frac{\iu\mathrm{e}^{\iu\alpha(\xi_{-1} - \varphi)} \mathrm{e}^{\iu\left(\lfloor\alpha\rfloor + \frac12\right)(\vartheta - \xi_{-1})}}{2\sin\left(\frac{\xi_{-1} - \vartheta}{2}\right)} - \frac{\iu\mathrm{e}^{\iu\alpha(\xi_1 - \varphi)} \mathrm{e}^{\iu\left(\lfloor\alpha\rfloor + \frac12\right)(\vartheta - \xi_1)}}{2\sin\left(\frac{\xi_1 - \vartheta}{2}\right)} = \frac{\sin(\alpha\pi)}{\sin\left(\frac{\varphi - \vartheta - \pi}{2}\right)}\mathrm{e}^{\iu\left(\lfloor\alpha\rfloor + \frac12\right)(\vartheta - \varphi + \pi)} .
			\label{eqMath38}
		\end{equation} Using this, the complete contribution gives us the outgoing wave:
		\begin{equation}
			\boldsymbol{\Psi}_{s,\boldsymbol{k}}^\mathrm{out}(r,\varphi) = \frac{F(\varphi-\vartheta)}{\sqrt{r}} \euler^{-\iu k r} \mathbf{u}_s(k,\varphi) ,
			\label{eqMath39}
		\end{equation} where the scattering function $F$ takes the following form:
		\begin{equation}
			F(\varphi - \vartheta) = \frac{\sin(\alpha\pi)\mathrm{e}^{\iu\left(\lfloor\alpha\rfloor + \frac12\right)(\vartheta - \varphi + \pi)}}{\sqrt{2\pi\iu k} \sin\left(\frac{\varphi - \vartheta - \pi}{2}\right)} .
			\label{eqMath40}
		\end{equation}
		
	\end{itemize} 
	
	So far, we have calculated the contribution of the saddle points, that is, the outgoing components of the asymptotic form. However, we also need to take into account the presence of poles in the integrand which appear at the point $\xi = \vartheta$ and equivalent points separated by multiples of $2\pi$. While deforming the contour as seen in Fig.\ \ref{figMath1}, we crossed one of these poles (exactly which one depends on the value of $\vartheta$ and $\varphi$). Consequently, we need to include the contribution of this pole as well using the residue of the following term in the integrand: 
	\begin{equation}
		\mathrm{Res}_{\xi = \vartheta} \left[\frac{1}{\sin\left(\frac{\xi - \vartheta}{2}\right)}\right] = 2 ,
		\label{eqMath41}
	\end{equation} the contribution can then be easily calculated:
	\begin{equation}
		\boldsymbol{\Psi}_{s,\boldsymbol{k}}^{\mathrm{in}}(r,\varphi) = \mathrm{e}^{\iu k r \cos(\varphi - \vartheta) - \iu\alpha(\varphi - \vartheta + \pi)} \mathbf{u}_{s}(\boldsymbol{k}) .
		\label{eqMath42}
	\end{equation} Considering all the contributions from Eqs.\ \eqref{eqMath35}, \eqref{eqMath39} and \eqref{eqMath42}, the asymptotic form of the trial solution reads:
	\begin{equation}
		\boldsymbol{\Psi}^{(+)}_{s,\boldsymbol{k}}(r,\varphi) \sim \boldsymbol{\Psi}_{s,\boldsymbol{k}}^{\mathrm{in}}(r,\varphi) + \boldsymbol{\Psi}_{s,\boldsymbol{k}}^{\mathrm{out}}(r,\varphi) ,
		\label{eqMath43}
	\end{equation} and thereby the final condition of $\boldsymbol{\Psi}^{(+)}_{s,\boldsymbol{k}}$ being the scattering state is also satisfied. Note that the asymptotic form given in Eq.\ \eqref{eqMath43} is only valid for $\varphi\in(-\pi,\pi)$, since for $\varphi = \pi$ the poles and the saddle points coincide and thereby the application of the method of steepest descent is not possible. In this special case, other approaches are available to obtain an asymptotic expansion; but it is irrelevant for our present purposes, and it shall be discussed elsewhere.
	
	\section{Probability Current Density}
	
	In the following section, we introduce the concept of probability density and probability current in general multiband electronic systems. These quantities are used to define the differential cross section, serving as the central observable of scattering theory.
	
	\subsection{General Derivation}
	
	To obtain the \textit{probability current density}, we need the time-dependent Schrödinger equation with respect to the Hamiltonian given in Eq.~(4) of the main text:
	\begin{equation}
		\iu\hbar \left(\partial_t\boldsymbol{\Psi}\right)(t) = \big(\hat{H}\boldsymbol{\Psi}\big)(t) ,
		\label{eqCross1}
	\end{equation} where we used the time-dependent state $\boldsymbol{\Psi}: \mathbb{R} \to \mathcal{H}$. The probability density of the electron position can be generally expressed as:
	\begin{equation}
		\varrho(t) = \sum_{a = 1}^D \Psi_a^*(t)\Psi_a(t),
		\label{eqCross2}
	\end{equation} where for some $1\le a\le D$ the functions $\Psi_a(t)\in L^2(\mathbb{R}^2)$ are the components of the vector $\boldsymbol{\Psi}(t)$. The time derivative of the probability density can be transformed using Eq.\ \eqref{eqCross1}:
	\begin{equation}
		\left(\partial_t\varrho\right)(t) = \sum_{a = 1}^D \partial_t\Psi_a^*(t)\Psi_a(t) + \Psi_a^*(t)\partial_t\Psi_a(t) = \frac{\iu}{\hbar} \sum_{a = 1}^D \big(\hat{H}\Psi_a\big)^*(t)\Psi_a(t) - \Psi_a^*(t)\big(\hat{H}\Psi_a\big)(t) .
		\label{eqCross3}
	\end{equation} After substitution of the concrete form of the Hamiltonian from Eq.~(4) of the main text:
	\begin{equation}
		\left(\partial_t\varrho\right)(t) = \frac{\iu}{\hbar} \sum_{a = 1}^D \sum_{b = 1}^D \sum_{i = 0}^I \sum_{j = 0}^J T_{ij}^{ab}\left[\big(\hat{\Pi}_x^i \hat{\Pi}_y^j \Psi_a \big)^*(t)\Psi_b(t) - \Psi_a^*(t)\big(\hat{\Pi}_x^i \hat{\Pi}_y^j \Psi_b \big)(t) \right] ,
		\label{eqCross4}
	\end{equation} where the matrix elements of the operators $\hat{T}_{ij}$ are denoted by $T_{ij}^{ab}\in\mathbb{C}$. Using the definition of the kinetic momentum operators $\hat{\Pi}_x$ and $\hat{\Pi}_y$ together with the product rule of differentiation we can bring Eq.\ \eqref{eqCross4} to the form of a \textit{continuity equation}:
	\begin{equation}
		\partial_t\varrho(t) + \left(\partial_x j_x\right)(t) + \left(\partial_y j_y\right)(t) = 0 ,
		\label{eqCross5}
	\end{equation} where the components $j_x$ and $j_y$ of the probability current density are defined as follows:
	\begin{subequations}
		\begin{align}
			j_x(t) &= \mathrm{Re}\left\{ \sum_{a = 1}^D \sum_{b = 1}^D \sum_{i = 0}^I \sum_{j = 0}^J \sum_{l = 0}^{i - 1} T_{ij}^{ab}\big(\hat{\Pi}_x^{i - l - 1} \hat{\Pi}_y^j \Psi_a \big)^*(t)\big(\hat{\Pi}_x^l\Psi_b \big)(t) \right\} , \label{eqCross6a} \\
			j_y(t) &= \mathrm{Re}\left\{ \sum_{a = 1}^D \sum_{b = 1}^D \sum_{i = 0}^I \sum_{j = 0}^J \sum_{l = 0}^{j - 1} T_{ij}^{ab}\big(\hat{\Pi}_y^{j  - l - 1} \Psi_a \big)^*(t) \big(\hat{\Pi}_y^{l} \hat{\Pi}_x^{i}\Psi_b\big)(t) \right\} . \label{eqCross6b}
		\end{align}
	\end{subequations} 
	
	\subsection{Examples: Plane Wave and Asymptotic Waves}
	
	In summary, Eqs.\ \eqref{eqCross6a} and \eqref{eqCross6b} define the general form of the probability current density. Apart from time-dependent real states, these formulae can also be applied to scattering states, i.e., distributions. 
	
	One such example is the probability current in the absence of a magnetic field with respect to a plane wave of the form written in Eq.~(2) of the main text. Then the operators $\hat{\Pi}_x$ and $\hat{\Pi}_y$ are replaced by $\hat{p}_x$ and $\hat{p}_y$ which act on plane waves by multiplicative factors $\hbar k_x$ and $\hbar k_y$, respectively. The resulting polynomials are then manifestly the partial derivatives of the dispersion relation with respect to $\hbar k_x$ and $\hbar k_y$, respectively, that is,
	\begin{equation}
		\boldsymbol{j}_{s,\boldsymbol{k}}(r,\varphi) = \boldsymbol{v}_s(k,\vartheta), \label{eqCross7}
	\end{equation} where $\boldsymbol{v}_s$ is the group velocity defined in Eq.~(7) of the main text. Rigorously, Eq.~\eqref{eqCross7} represents equality only component-wise since the two vector fields lie on different manifolds. Nevertheless, this conclusion is extremely useful.
	
	Another example is the current density in the presence of a magnetic field with respect to the asymptotic components given in Eqs.\ \eqref{eqMath35}, \eqref{eqMath39} and \eqref{eqMath42}. These can be calculated using Eqs.\ \eqref{eqCross7} and \eqref{eqMath27a}:
	\begin{subequations}
		\label{eqCross8}
		\begin{align}
			\boldsymbol{j}_{s,\boldsymbol{k}}^\mathrm{in}(r,\varphi) &= \boldsymbol{v}_s(k,\vartheta) , \label{eqCross8a} \\
			\boldsymbol{j}_{s,\boldsymbol{k}}^\mathrm{out}(r,\varphi) &= \frac{|F(\varphi - \vartheta)|^2}{r} \boldsymbol{v}_s(k,\varphi) + O\big(r^{-3/2}\big) . \label{eqCross8b}
		\end{align}
	\end{subequations} The results agree with Eq.~(10) of the main text, which is a crucial identity towards the determination of the differential cross section.
	
	
	\section{Details of the Applications}
	
	In the following section, the application of our general theory to specific multiband electronic systems is presented. Apart from the more detailed derivation of the scattering states given in Table I of the main text, we also provide an insightful visualization of the wave functions.
	
	\subsection{Two-Dimensional Electron Gas}
	\label{graphene:supp_sec}
	
	The first example to be discussed is the \emph{two-dimensional electron gas}. Such a system can appear in GaAs-AlGaAs heterojunctions where the difference of Fermi energies causes a rearrangement in the electron distribution producing an electrostatic potential. This electric field confines other electrons into a thin two-dimensional layer at the interface of the two semiconductors producing a quasi-two-dimensional conducting layer \cite{datta_1995}. The dynamics in this system can be described by a two-dimensional model of free particles with some effective mass differing from the mass of the electron. The Aharonov--Bohm effect in an analogous system of free non-relativistic particles was investigated before by Aharonov and Bohm, and also by Berry \cite{Aharonov-Bohm:cikk,Berry_1980,Berry_Chambers_1980}. In the following, we aim to reproduce their results using our newly developed methods.
	
	%\subsubsection{Hamiltonian Operator}
	%\label{subsec311}
	
	The Hilbert space corresponding to the two-dimensional electron gas is simply $\mathcal{H} = L^2(\mathbb{R}^2,\mathbb{C})$, that is, there is no inner degree of freedom present ($D=1$). Note that although the electron has a spin, it is not relevant in our case as it has no effect on the dynamics. The Hamiltonian operator $\hat{H}: \mathcal{D}_H \to \mathcal{H}$ is given as a quadratic polynomial of the momentum operators:
	\begin{equation}
		\hat{H} = \frac{1}{2M} \left(\hat{p}_x^2 + \hat{p}_y^2\right) ,
		\label{eqIso1}
	\end{equation} where $M$ is the effective mass of the electrons. 
	
	%\subsubsection{Band Structure and its Properties}
	%\label{subsec312}
	
	The band structure corresponding to the Hamiltonian in Eq.\ \eqref{eqIso1} consists of a single band which is given in polar coordinates as:
	\begin{equation}
		E(k,\vartheta) = \frac{\hbar^2 k^2}{2M} .
		\label{eqIso2}
	\end{equation} As expected, the isotropy of the system is manifested in the shape of the band structure: the constant energy curves are circles for all values of the energy. The momentum space eigenvectors need to be chosen such that one of its components is independent of $\vartheta$. In this case, there is only one possible choice up to a constant multiplier:
	\begin{equation}
		\mathbf{u}(k,\vartheta) = 1 .
		\label{eqIso3}
	\end{equation}
	
	%\begin{figure}[hbt]
	%\centering
	%\vspace*{-20pt}
	%\includegraphics[scale=0.833]{Spinless_Bands1.pdf}\hspace{10pt}
	%\includegraphics[scale=0.833]{Spinless_Bands2.pdf}
	%\caption{Surface plot (on the left) and contour plot (on the right) corresponding to the band structure of the two-dimensional electron gas in Equation \eqref{eqIso4}. Natural length and energy units $d_0$ and $E_0$ were used to make the scales dimensionless.}
	%\label{figIso1}
	%\end{figure}
	
	The group velocity vector field is easily determined from Eq.\ \eqref{eqIso2} by taking its gradient with respect to $\hbar\boldsymbol{k}$. The results are the following:
	\begin{subequations}
		\begin{align}
			v_k(k,\vartheta) &= \frac{\hbar k}{M} , 
			\label{eqIso4a} \\
			v_\vartheta(k,\vartheta) &= 0 . 
			\label{eqIso4b}
		\end{align} 
	\end{subequations} It is clearly seen that the radial group velocity is everywhere positive (except at the origin), thereby we can call the single band of this model an \emph{electron-like band}. As we have seen before, this observation is important from the point of view of the scattering states.
	
	%\subsubsection{Probability Current}
	
	A further important quantity is the probability density of the electron position corresponding to an arbitrary state $\Psi\in\mathcal{H}$. This can be written as a special case of Eq.\ \eqref{eqCross2} for this single-band system:
	\begin{equation}
		\varrho = \Psi^* \Psi .
		\label{eqIso5}
	\end{equation} The probability current density on the other hand depends on the Hamiltonian in Eq.\ \eqref{eqIso1} as well. Applying the results of Eqs.\ \eqref{eqCross6a} and \eqref{eqCross6b} we find:
	\begin{subequations}
		\begin{align}
			j_x &= \frac{1}{M}~\mathrm{Re}\left[\Psi^* \big(\hat{\Pi}_x \Psi\big) \right] , \label{eqIso6a} \\
			j_y &= \frac{1}{M}~\mathrm{Re}\left[\Psi^* \big(\hat{\Pi}_y \Psi\big) \right] . \label{eqIso6b}
		\end{align}
	\end{subequations}
	
	%\subsubsection{Scattering States}
	%\label{subsec314}
	
	With all the ingredients collected, now Eq.~(5) of the main text can be applied to calculate the scattering states. Since the wave function has a single component in this case, the general formula reduces to Eq.~\eqref{eqMath5a} of this Supplemental Material. After direct substitution, we can further apply the Schäfli--Sommerfeld integral formula of the Bessel functions of the first kind \cite{Grads:book} to simplify the expressions. The final result is the following:
	\begin{equation}
		\Psi^{(+)}_{\boldsymbol{k}}(r,\varphi) = \sum_{m=-\infty}^\infty (-\iu)^{|m+\alpha|} J_{|m+\alpha|}(k r) \euler^{\iu m(\varphi - \vartheta + \pi)} .
		\label{eqIso7}
	\end{equation} Setting $\vartheta = \pi$ this is exactly the solution obtained by Aharonov and Bohm in their original paper \cite{Aharonov-Bohm:cikk}; thus, we managed to reproduce their results as hoped. This observation gives strong support to our novel method.
	
	\begin{figure}[hbt]
		\begin{subfigure}{0.49\linewidth}
			\centering
			\includegraphics[scale=0.833]{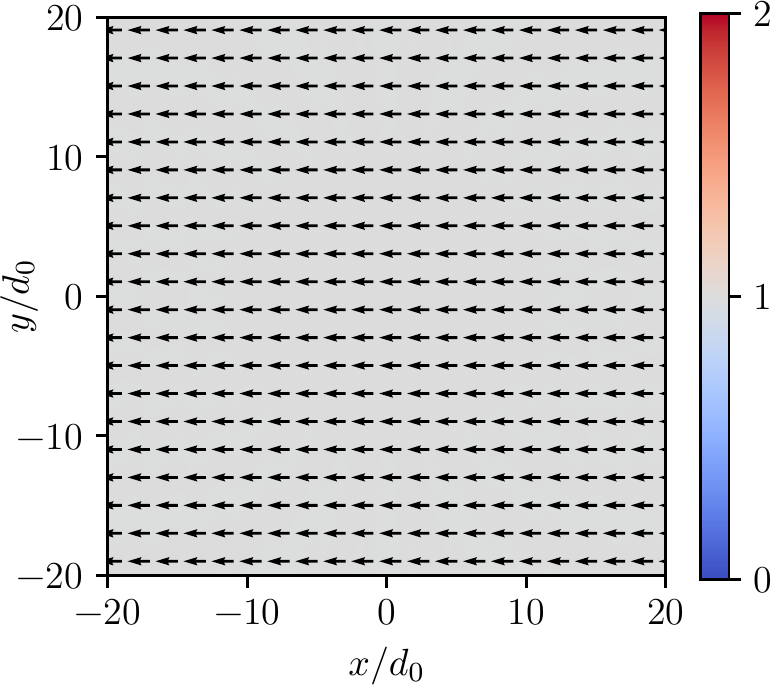}
			\caption{$\alpha = 0$}
			\label{figIso1a}
		\end{subfigure}
		\begin{subfigure}{0.49\linewidth}
			\centering
			\includegraphics[scale=0.833]{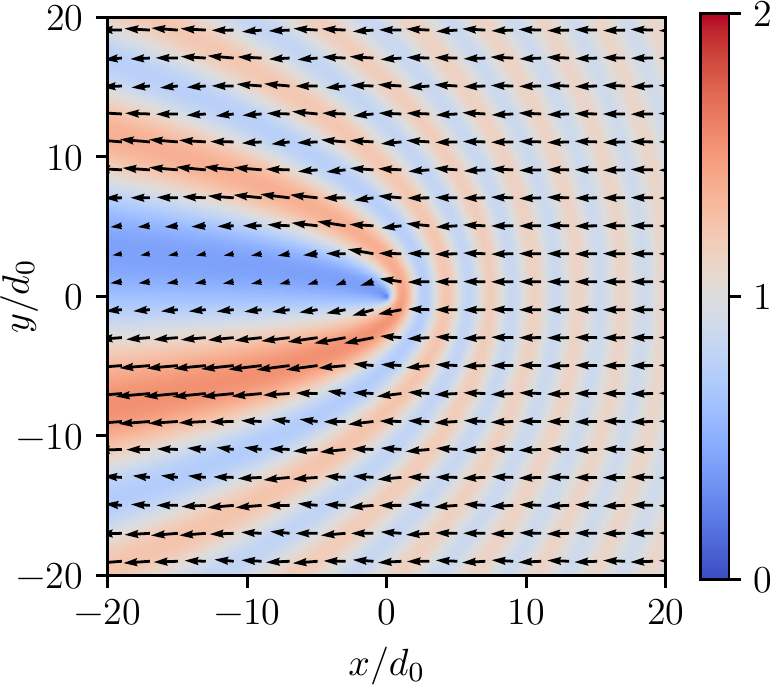}
			\caption{$\alpha = 0.2$}
			\label{figIso1b}
		\end{subfigure}
		\begin{subfigure}{0.49\linewidth}
			\centering
			\includegraphics[scale=0.833]{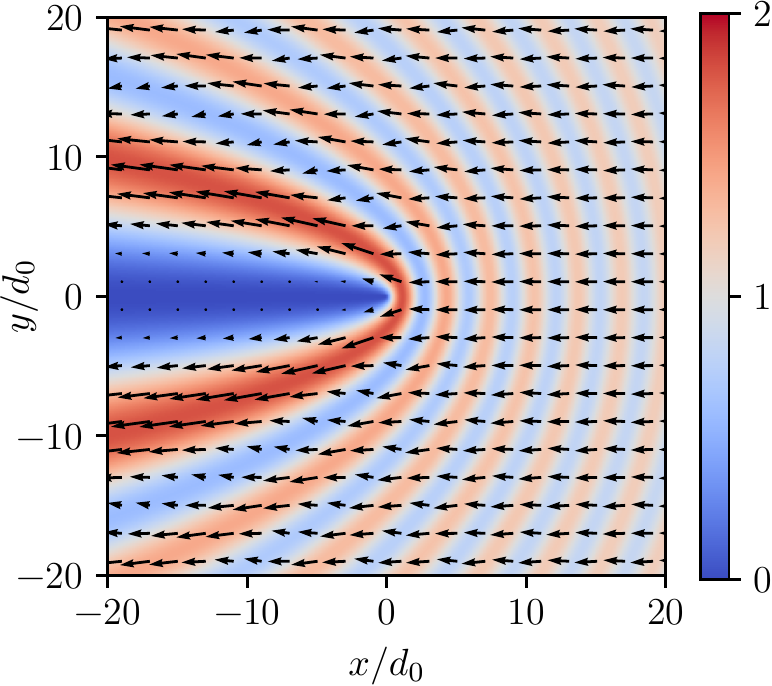}
			\caption{$\alpha = 0.5$}
			\vspace*{5pt}
			\label{figIso1c}
		\end{subfigure}
		\begin{subfigure}{0.49\linewidth}
			\centering
			\includegraphics[scale=0.833]{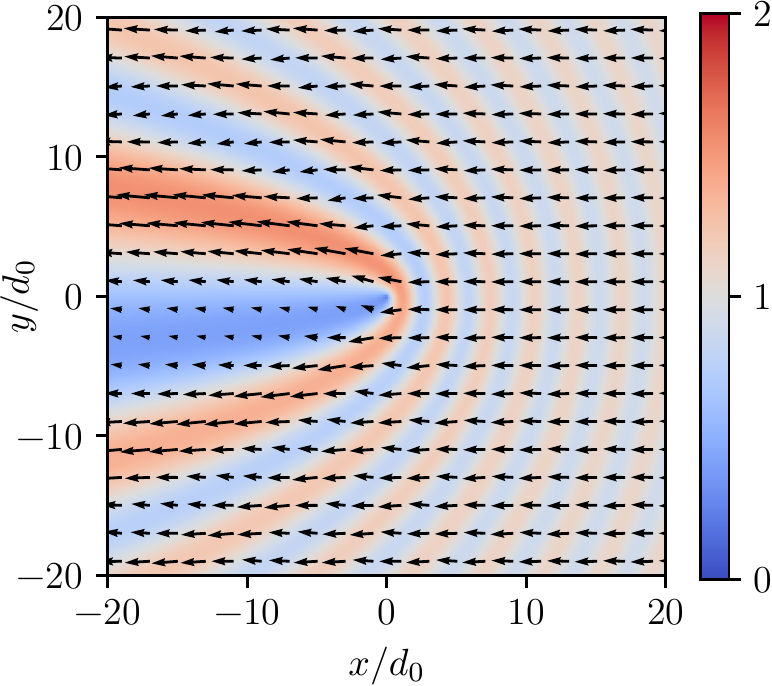}
			\caption{$\alpha = 0.8$}
			\vspace*{5pt}
			\label{figIso1d}
		\end{subfigure}
		\caption{Scattering states corresponding to the Aharonov--Bohm effect in a two-dimensional electron gas. The probability density $\varrho$ (represented by the colors) and current density $\boldsymbol{j}$ (represented by the arrows) are computed for $kd_0 = 1$ (where $d_0$ is a natural length unit) and different values of the parameter $\alpha$.}
		\label{figIso1}
	\end{figure}
	
	To gain a deeper understanding of the scattering states, we can calculate the corresponding probability density and current density using Eqs.\ \eqref{eqIso5}, \eqref{eqIso6a} and \eqref{eqIso6b}. The results of the numerical calculations are shown in Fig.\ \ref{figIso1}, let us now examine them in detail. In the $\alpha=0$ case shown in Fig.\ \ref{figIso1a}, a simple plane wave can be seen in agreement with our analytical calculations done in Eq.\ \eqref{eqMath30}. However, if $\alpha$ is increased, a non-trivial scattering occurs, see Fig.\ \ref{figIso1b}. Further increasing the flux, the scattering is maximal for $\alpha = 0.5$, see Fig.\ \ref{figIso1c}. After this value, a weakening is observed, see Fig.\ \ref{figIso1d}, and eventually for integer $\alpha=1$, one gets back the same result as for $\alpha=0$. Furthermore, for any integer $\alpha$ value the same plane wave is recovered (up to a complex phase): this periodicity indicates the strictly quantum nature of the Aharonov--Bohm effect. Additionally, the system has an interesting symmetry: reflection with respect to the $x$ axis and a simultaneous $\alpha \to -\alpha$ transformation (the latter is needed due to the \textit{axial vector} behavior of the magnetic field). This symmetry together with the periodicity property implies that the scattering states corresponding to any $\alpha$ and $1 - \alpha$ are the reflections of each other. Specifically, states belonging to half-integer values of the dimensionless flux are reflection invariant, see Fig.\ \ref{figIso1c}.
	
	\subsection{Monolayer Graphene}
	\label{graphene:supp_sec}
	
	The second example to be discussed is the \emph{monolayer graphene}, that is, the two-dimensional honeycomb lattice of carbon atoms \cite{Novoselov2005,Zhang2005,DiVincenzo_Mele_PRB_29_1685:ref,RevModPhys.81.109}. In this system, the band structure contains so-called Dirac cones, that is, in a close neighborhood of points $K$ and $K'$ of the Brillouin zone the dispersion relation has a conic behavior. As a consequence, the low-energy behavior of electrons in graphene is similar to that of massless spin-$1/2$ relativistic particles which gives us an opportunity to use an effective description in this regime. More precisely, the so-called \textit{envelope function approximation} can be used which states that sharply peaked wave packets around the $K$ and $K'$ points obey an effective Dirac--Weyl dynamics. The Aharonov--Bohm effect in the analogous system of relativistic particles was investigated before by Alford, Wilczek, Gerbert and Hagen \cite{Wilczek_PhysRevLett.62.1071,Gerbert_PhysRevD.40.1346,Hagen_PhysRevLett.64.503,Hagen_PhysRevD.42.3524}.  In the following, we aim to reproduce their results using our newly developed methods.
	
	%\subsubsection{Hamiltonian Operator}
	%\label{subsec321}
	
	The Hilbert space corresponding to monolayer graphene is $\mathcal{H} = L^2(\mathbb{R}^2,\mathbb{C})\otimes\mathbb{C}^2$, that is, there is a two-state inner degree of freedom ($D=2$) corresponding to the two sublattices of the crystal. The Hamiltonian operator $\hat{H}: \mathcal{D}_H \to \mathcal{H}$ is given as a linear polynomial of the momentum operators:
	\begin{equation}
		\hat{H} = v \left(\hat{p}_x\otimes\hat{\sigma}_x + \hat{p}_y\otimes\hat{\sigma}_y\right) ,
		\label{eqIso8}
	\end{equation} where $v$ is an effective velocity parameter and 
	\begin{equation}
		\hat{\sigma}_x = \begin{pmatrix}
			~0~ & ~1~ \\ ~1~ & ~0~
		\end{pmatrix},~~~~~\hat{\sigma}_y = \begin{pmatrix}
			~0~ & -\mathrm{i}~ \\ ~\mathrm{i}~ & ~0~
		\end{pmatrix},~~~~~\hat{\sigma}_z = \begin{pmatrix}
			~1~ & ~0~ \\ ~0~ & -1~
		\end{pmatrix}.
		\label{eqIso9}
	\end{equation} are the \textit{Pauli operators} given in matrix representation. 
	
	%\subsubsection{Band Structure and its Properties}
	%\label{subsec322}
	
	The band structure corresponding to the Hamiltonian in Eq.\ \eqref{eqIso8} consists of two bands with $s\in\{-1,1\}$ which are given in polar coordinates as:
	\begin{equation}
		E_s(k,\vartheta) = s v \hbar k .
		\label{eqIso10}
	\end{equation} As expected, the isotropy of the system is manifested in the shape of the band structure: the constant energy curves are circles for all values of the energy. The momentum space eigenvectors need to be chosen such that one of its components is independent of $\vartheta$. We can choose this to be the upper component:
	\begin{equation}
		\mathbf{u}_s(k,\vartheta) = \frac{1}{\sqrt2} \begin{pmatrix}
			1 \\ s \euler^{\iu\vartheta}
		\end{pmatrix} .
		\label{eqIso11}
	\end{equation} As was detailed in the \textsl{Condition (i): Convergence and Single-Valuedness} subsection, this choice corresponds to the upper component of the scattering state being regular at the origin. In fact, Hagen has shown that this is the boundary condition following from taking the $R\to 0$ limit of a finite radius solenoid if $\alpha>0$ \cite{Hagen_PhysRevLett.64.503}. In the $\alpha<0$ case, the lower component must be regular. However, in the following, we shall stick to the postulated boundary condition of the upper component being regular in agreement with the vector given in Eq.\ \eqref{eqIso11}.
	
	%\begin{figure}[hbt]
	%\centering
	%\vspace*{-20pt}
	%\includegraphics[scale=0.833]{Graphene_Bands1.pdf}\hspace{10pt}
	%\includegraphics[scale=0.833]{Graphene_Bands2.pdf}
	%\caption{Surface plot (on the left) and contour plot (on the right) corresponding to the band structure of the monolayer graphene in Equation \eqref{eqIso17}.  Natural length and energy units $d_0$ and $E_0$ were used to make the scales dimensionless.}
	%\label{figIso3}
	%\end{figure}
	
	The group velocity vector field is easily determined from Eq.\ \eqref{eqIso10} by taking its gradient with respect to $\hbar\boldsymbol{k}$. The results are the following:
	\begin{subequations}
		\begin{align}
			v_{s,k}(k,\vartheta) &= sv , 
			\label{eqIso12a} \\
			v_{s,\vartheta}(k,\vartheta) &= 0 . 
			\label{eqIso12b}
		\end{align} 
	\end{subequations} It is clearly seen that the radial group velocity is either everywhere positive or everywhere negative depending on the band index $s$. Based on this, we can call the band with $s=1$ \emph{electron-like}, and the band with $s=-1$ \emph{hole-like}. 
	
	%\subsubsection{Probability Current}
	%\label{subsec323}
	
	A further important quantity is the probability density of the electron position corresponding to an arbitrary state $\boldsymbol{\Psi} = \left(\Psi_1,\Psi_2\right) \in \mathcal{H}$. This can be written as a special case of Eq.\ \eqref{eqCross2} for this two-band system:
	\begin{equation}
		\varrho = \Psi_1^* \Psi_1 + \Psi_2^* \Psi_2 .
		\label{eqIso13}
	\end{equation} The probability current density on the other hand depends on the Hamiltonian in Eq.\ \eqref{eqIso8} as well. Applying the results of Eqs.\ \eqref{eqCross6a} and \eqref{eqCross6b}, we find:
	\begin{subequations}
		\begin{align}
			j_x &= 2v~\mathrm{Re}\left(\Psi_1^*\Psi_2\right), \label{eqIso14a} \\
			j_y &= 2v~\mathrm{Im}\left(\Psi_1^*\Psi_2\right). \label{eqIso14b}
		\end{align}
	\end{subequations} 
	
	%\subsubsection{Scattering States}
	%\label{subsec324}
	
	With all the ingredients collected, now Eq.~(5) of the main text can be applied to calculate the scattering states. The integral representation of the Bessel functions can again be used \cite{Grads:book}, the final result for the electron-like band with $s=1$ is
	\begin{equation}
		\boldsymbol{\Psi}^{(+)}_{1,\boldsymbol{k}}(r,\varphi) = \sum_{m=-\infty}^\infty \frac{(-\iu)^{|m+\alpha|} \euler^{\iu m (\varphi - \vartheta + \pi)}}{\sqrt2} \begin{pmatrix} J_{|m+\alpha|}(k r) \\ \iu \epsilon(m + \alpha) J_{|m+\alpha| + \epsilon(m+\alpha)}(k r) \euler^{\iu\varphi} \end{pmatrix} ,
		\label{eqIso15}
	\end{equation} whereas for the hole-like band with $s=-1$ is
	\begin{equation}
		\boldsymbol{\Psi}^{(+)}_{-1,\boldsymbol{k}}(r,\varphi) = \sum_{m=-\infty}^\infty \frac{\iu^{|m+\alpha|} \euler^{\iu m (\varphi - \vartheta + \pi)}}{\sqrt2} \begin{pmatrix} J_{|m+\alpha|}(k r) \\ -\iu \epsilon(m + \alpha) J_{|m+\alpha| + \epsilon(m+\alpha)}(k r) \euler^{\iu\varphi} \end{pmatrix} .
		\label{eqIso16}
	\end{equation} Setting $\vartheta = \pi$ this is exactly the solution obtained by Alford, Wilczek, Gerbert, and Hagen in their papers \cite{Wilczek_PhysRevLett.62.1071,Gerbert_PhysRevD.40.1346,Hagen_PhysRevLett.64.503}; thus, we managed to reproduce their results as hoped. This observation gives further support to our novel method.
	
	\begin{figure}[!h]
		\begin{subfigure}{0.49\linewidth}
			\centering
			\includegraphics[scale=0.833]{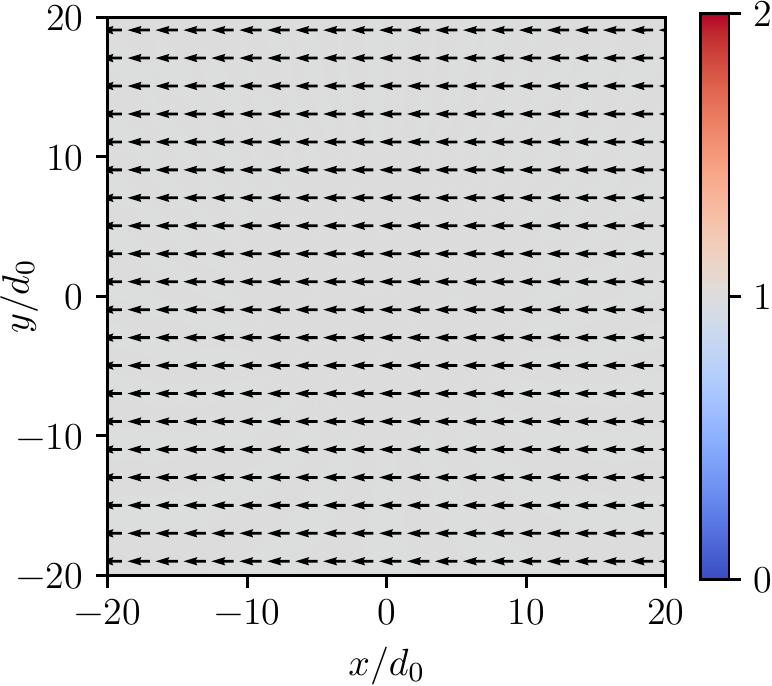}
			\caption{$s=1$, $\alpha = 0$}
			\vspace*{5pt}
			\label{figIso2a}
		\end{subfigure}
		\begin{subfigure}{0.49\linewidth}
			\centering
			\includegraphics[scale=0.833]{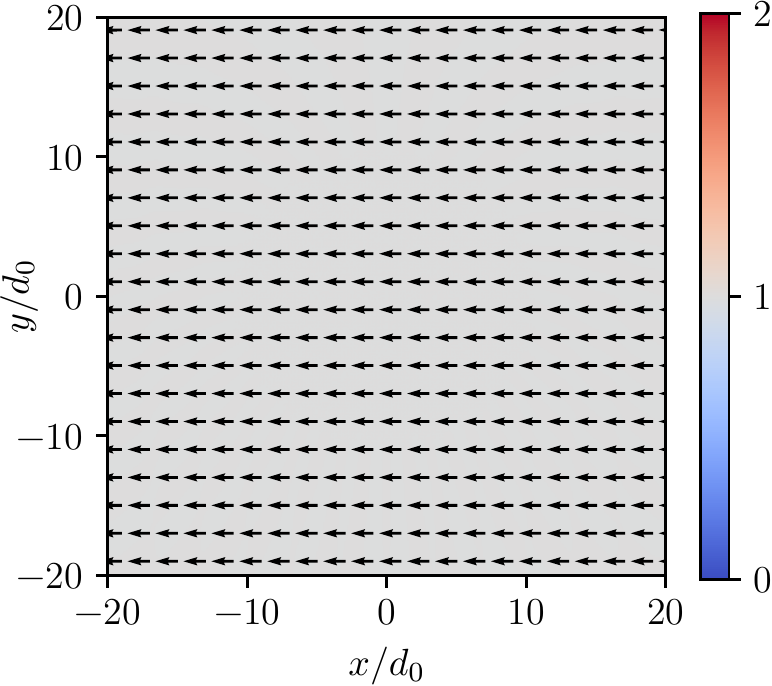}
			\caption{$s=-1$, $\alpha = 0$}
			\vspace*{5pt}
			\label{figIso2b}
		\end{subfigure}
		\begin{subfigure}{0.49\linewidth}
			\centering
			\includegraphics[scale=0.833]{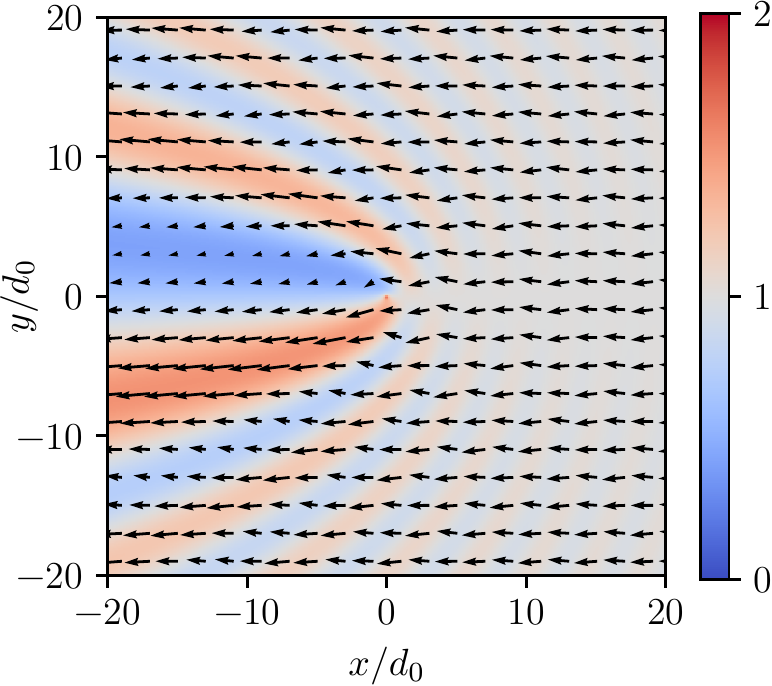}
			\caption{$s=1$, $\alpha = 0.2$}
			\vspace*{5pt}
			\label{figIso2c}
		\end{subfigure}
		\begin{subfigure}{0.49\linewidth}
			\centering
			\includegraphics[scale=0.833]{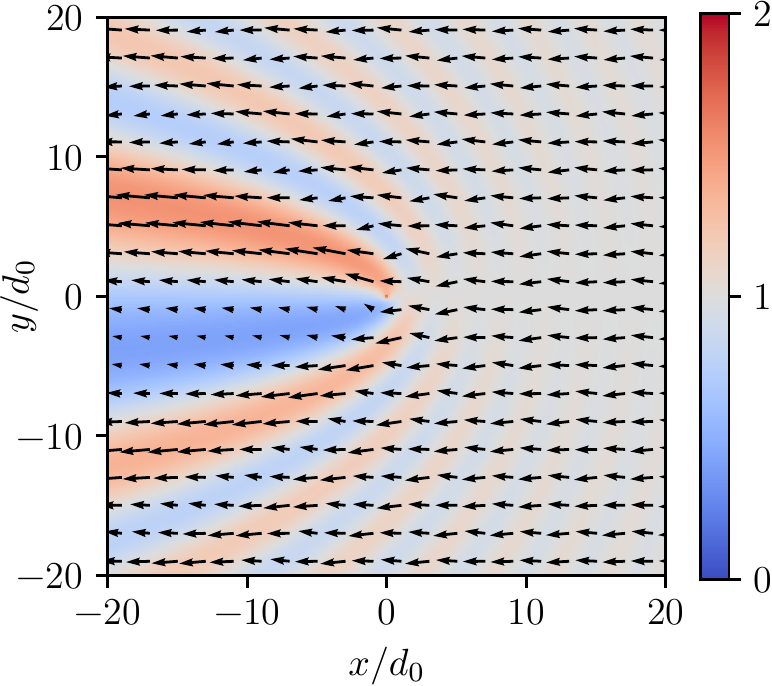}
			\caption{$s=-1$, $\alpha = 0.2$}
			\vspace*{5pt}
			\label{figIso2d}
		\end{subfigure}
		\begin{subfigure}{0.49\linewidth}
			\centering
			\includegraphics[scale=0.833]{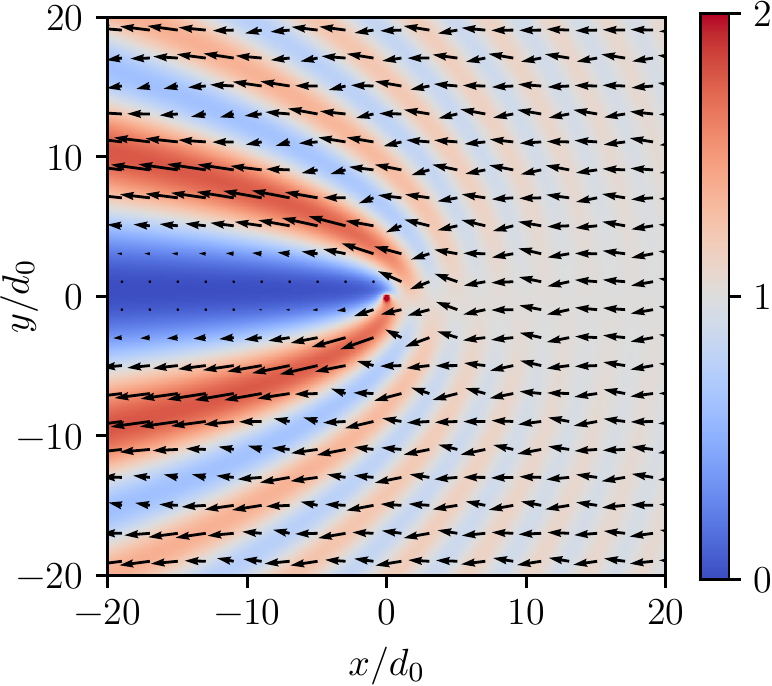}
			\caption{$s=1$, $\alpha = 0.5$}
			\vspace*{0pt}
			\label{figIso2e}
		\end{subfigure}
		\begin{subfigure}{0.49\linewidth}
			\centering
			\includegraphics[scale=0.833]{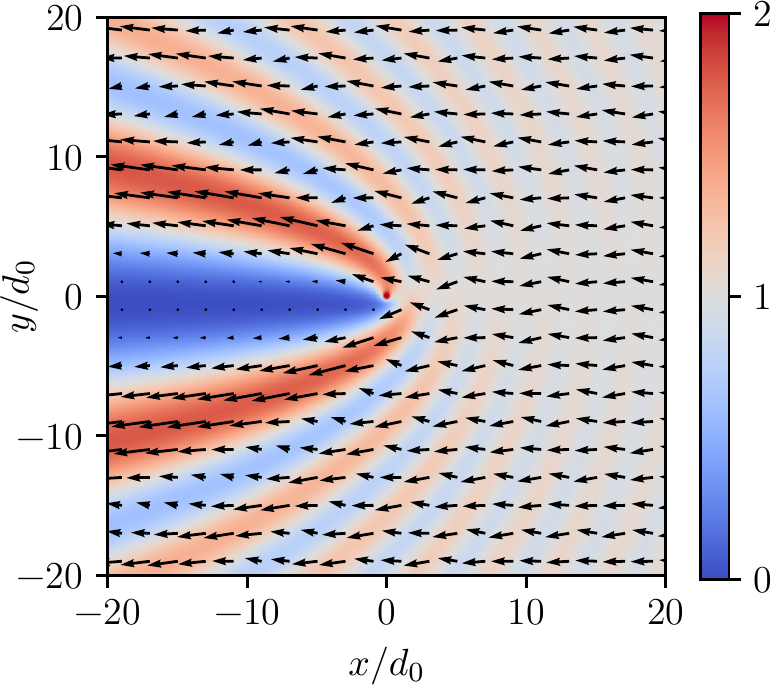}
			\caption{$s=-1$, $\alpha = 0.5$}
			\vspace*{0pt}
			\label{figIso2f}
		\end{subfigure}
	\end{figure}
	
	\begin{figure}[!h]
		\ContinuedFloat
		\begin{subfigure}{0.49\linewidth}
			\centering
			\includegraphics[scale=0.833]{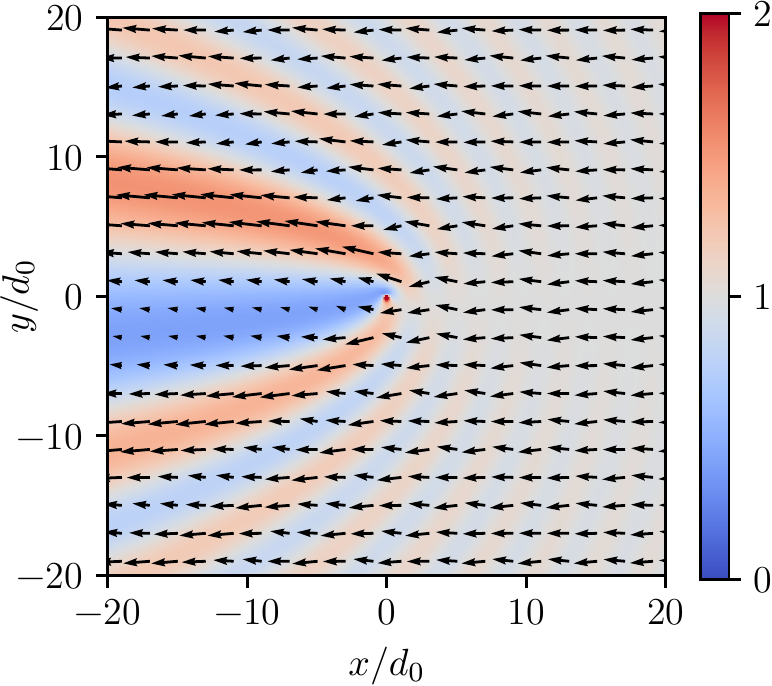}
			\caption{$s=1$, $\alpha = 0.8$}
			\vspace*{5pt}
			\label{figIso2g}
		\end{subfigure}
		\begin{subfigure}{0.49\linewidth}
			\centering
			\includegraphics[scale=0.833]{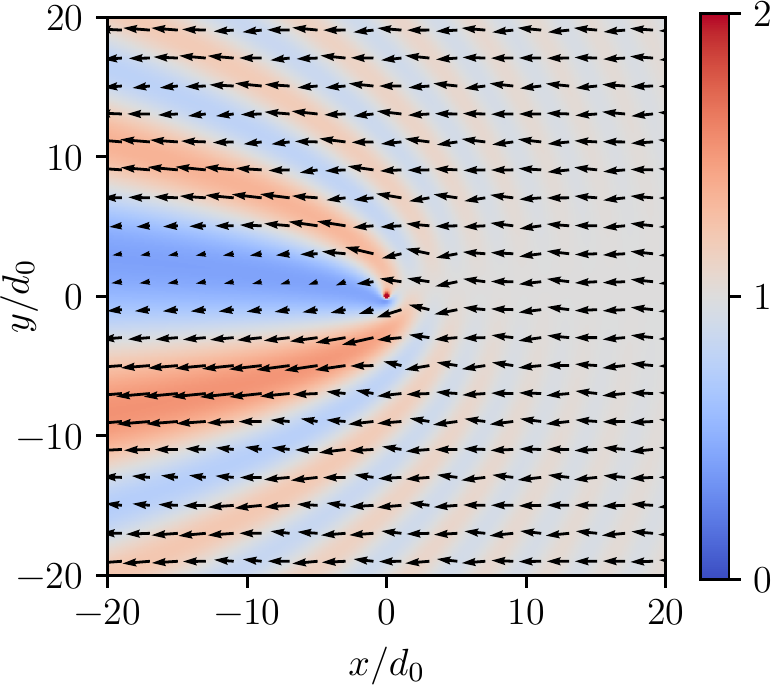}
			\caption{$s=-1$, $\alpha = 0.8$}
			\vspace*{5pt}
			\label{figIso2h}
		\end{subfigure}
		\caption{Scattering states corresponding to the Aharonov--Bohm effect in monolayer graphene. The probability density $\varrho$ (represented by the colors) and current density $\boldsymbol{j}$ (represented by the arrows) are computed for $kd_0 = 1$ (where $d_0$ is a natural length unit) and different values of the parameters $s$ and $\alpha$.}
		\label{figIso2}
	\end{figure}
	
	The probability density and current density corresponding to these scattering states can again be numerically evaluated using Eqs.\ \eqref{eqIso13}, \eqref{eqIso14a} and \eqref{eqIso14b}, the results are shown in Fig.\ \ref{figIso2}. The results are quite similar to the case of the two-dimensional electron gas in the previous subsection, there are only a few differences worth mentioning. First, we can see that the scattering states corresponding to the two bands differ from each other: the alternation of colors is rather different in Fig.\  \ref{figIso2c} and \ref{figIso2d} for example. Second, there is a singularity at the origin not present before which can be observed in the form of a small red dot, for instance in Fig.\ \ref{figIso2e}. This corresponds to the fact that both components of the scattering states cannot be regular at the same time as pointed out by Gerbert \cite{Gerbert_PhysRevD.40.1346}. We chose the upper component as regular which results in the lower component being singular.
	
	
	\subsection{Bilayer Graphene}
	\label{bilayer_graphene:supp_sec}
	
	The third example to be discussed is the \emph{bilayer graphene}, that is, two layers of graphene on top of each other in a shifted manner \cite{Novoselov_Hall:ref,mccann:086805}. In the usual tight-binding description taking into account the nearest neighbor interactions inter- and intra-layer, the band structure of this material consists of four parabolic bands. Two of these touch at the Fermi energy, and the other two are shifted above and below that. Thus, in the low-energy regime, one can consider only the effect of the low-lying bands and neglect the other pair. This results in an effective two-band model of bilayer graphene which is frequently used in the literature. To the best of our knowledge, the Aharonov--Bohm effect in this system has not been investigated before. In the following, we aim to do so using our newly developed methods.
	
	%\subsubsection{Hamiltonian Operator}
	%\label{subsec331}
	
	The Hilbert space corresponding to bilayer graphene is $\mathcal{H} = L^2(\mathbb{R}^2,\mathbb{C})\otimes\mathbb{C}^2$, that is, there is a two-state inner degree of freedom ($D=2$) corresponding to the two sublattices of the crystal. The Hamiltonian operator $\hat{H}: \mathcal{D}_H \to \mathcal{H}$ is given as a quadratic polynomial of the momentum operators:
	\begin{equation}
		\hat{H} = - \frac{1}{2M} \left[\left(\hat{p}_x^2 - \hat{p}_y^2\right)\otimes\hat{\sigma}_x + 2\hat{p}_x\hat{p}_y\otimes\hat{\sigma}_y\right] ,
		\label{eqIso17}
	\end{equation} where $M$ is an effective mass parameter, and $\hat{\sigma}_x$, $\hat{\sigma}_y$ and $\hat{\sigma}_z$ are the Pauli operators defined in Eq.\ \eqref{eqIso9}. 
	
	%\subsubsection{Band Structure and its Properties}
	%\label{subsec332}
	
	The band structure corresponding to the Hamiltonian in Eq.\ \eqref{eqIso17} consists of two bands with $s\in\{-1,1\}$ which are given in polar coordinates as:
	\begin{equation}
		E_s(k,\vartheta) = s \frac{\hbar^2 k^2}{2M} .
		\label{eqIso18}
	\end{equation} As expected, the isotropy of the system is manifested in the shape of the band structure: the constant energy curves are circles for all values of the energy. The momentum space eigenvectors need to be chosen such that one of its components is independent of $\vartheta$. We can choose this to be the upper component:
	\begin{equation}
		\mathbf{u}_s(k,\vartheta) = \frac{1}{\sqrt2} \begin{pmatrix} 1 \\ -s \euler^{2\iu\vartheta} \end{pmatrix} .
		\label{eqIso19}
	\end{equation}
	
	%\begin{figure}[hbt]
	%\centering
	%\vspace*{-20pt}
	%\includegraphics[scale=0.833]{Bilayer_Bands1.pdf}\hspace{10pt}
	%\includegraphics[scale=0.833]{Bilayer_Bands2.pdf}
	%\caption{Surface plot (on the left) and contour plot (on the right) corresponding to the band structure of the bilayer graphene in Equation \eqref{eqIso38}. Natural length and energy units $d_0$ and $E_0$ were used to make the scales dimensionless.}
	%\label{figIso8}
	%\end{figure}
	
	The group velocity vector field is easily determined from Eq.\ \eqref{eqIso18} by taking its gradient with respect to $\hbar\boldsymbol{k}$. The results are the following:
	\begin{subequations}
		\begin{align}
			v_{s,k}(k,\vartheta) &= s \frac{\hbar k}{M} , 
			\label{eqIso20a} \\
			v_{s,\vartheta}(k,\vartheta) &= 0 . 
			\label{eqIso20b}
		\end{align} 
	\end{subequations} It is clearly seen that the radial group velocity is either everywhere positive or everywhere negative (except at the origin) depending on the band index $s$. Based on this, we can call the band with $s=1$ electron-like, and the band with $s=-1$ hole-like.
	
	%\subsubsection{Probability Current}
	
	A further important quantity is the probability density of the electron position corresponding to an arbitrary state $\boldsymbol{\Psi} = \left(\Psi_1,\Psi_2\right) \in \mathcal{H}$. This can be written as a special case of Eq.\ \eqref{eqCross2} for this two-band system:
	\begin{equation}
		\varrho = \Psi_1^* \Psi_1 + \Psi_2^* \Psi_2 .
		\label{eqIso21}
	\end{equation} The probability current density on the other hand depends on the Hamiltonian in Eq.\ \eqref{eqIso17} as well. Applying the results of Eqs.\ \eqref{eqCross6a} and \eqref{eqCross6b} we find:
	\begin{subequations}
		\begin{align}
			j_x &= -\frac{1}{M}~\mathrm{Re}\left[\Psi_1^*\big(\hat{\Pi}_x\Psi_2\big) + \Psi_2^*\big(\hat{\Pi}_x\Psi_1\big) - \iu \Psi_1^*\big(\hat{\Pi}_y \Psi_2\big) + \iu \Psi_2^*\big(\hat{\Pi}_y \Psi_1\big) \right] , 
			\label{eqIso22a} \\
			j_y &= \frac{1}{M}~\mathrm{Re}\left[\Psi_1^*\big(\hat{\Pi}_y\Psi_2\big) + \Psi_2^*\big(\hat{\Pi}_y\Psi_1\big) + \iu \Psi_1^*\big(\hat{\Pi}_x \Psi_2\big) - \iu \Psi_2^*\big(\hat{\Pi}_x \Psi_1\big) \right] . 
			\label{eqIso22b}
		\end{align}
	\end{subequations}
	
	%\subsubsection{Scattering States}
	
	With all the ingredients collected, now Eq.~(5) of the main text can be applied to calculate the scattering states. The integral representation of the Bessel functions can again be used \cite{Grads:book}, the final result for the electron-like band with $s=1$ is
	\begin{equation}
		\boldsymbol{\Psi}^{(+)}_{1,\boldsymbol{k}}(r,\varphi) = \sum_{m=-\infty}^\infty \frac{(-\iu)^{|m+\alpha|} \euler^{\iu m (\varphi - \vartheta + \pi)}}{\sqrt2} \begin{pmatrix} J_{|m+\alpha|}(k r) \\ J_{|m+\alpha| + 2\epsilon(m+\alpha)}(k r) \euler^{2\iu\varphi} \end{pmatrix} ,
		\label{eqIso23}
	\end{equation} whereas for the hole-like band with $s=-1$ is
	\begin{equation}\boldsymbol{\Psi}^{(+)}_{-1,\boldsymbol{k}}(r,\varphi) = \sum_{m=-\infty}^\infty \frac{\iu^{|m+\alpha|} \euler^{\iu m (\varphi - \vartheta + \pi)}}{\sqrt2} \begin{pmatrix} J_{|m+\alpha|}(k r) \\ -J_{|m+\alpha| + 2\epsilon(m+\alpha)}(k r) \euler^{2\iu\varphi} \end{pmatrix} ,
		\label{eqIso24}
	\end{equation} To the best of our knowledge, these results cannot be found in the literature.
	
	The probability density and current density corresponding to these scattering states can again be numerically evaluated utilizing Eqs.\ \eqref{eqIso21}, \eqref{eqIso22a} and \eqref{eqIso22b}, the results are shown in Fig.\ \ref{figIso3}. These are quite similar to the case of monolayer graphene discussed in the previous subsection.
	
	\begin{figure}[!h]
		\begin{subfigure}{0.49\linewidth}
			\centering
			\includegraphics[scale=0.833]{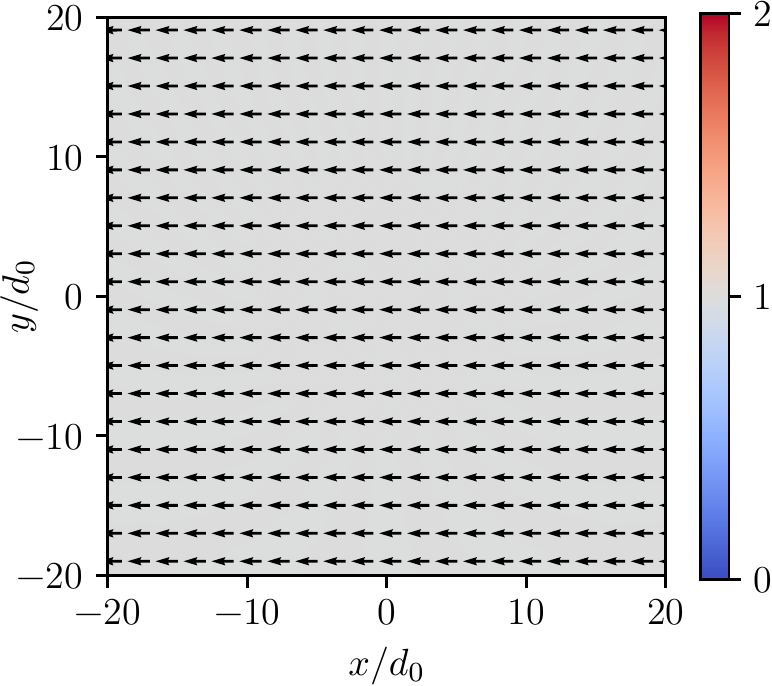}
			\caption{$s=1$, $\alpha = 0$}
			\vspace*{0pt}
			\label{figIso3a}
		\end{subfigure}
		\begin{subfigure}{0.49\linewidth}
			\centering
			\includegraphics[scale=0.833]{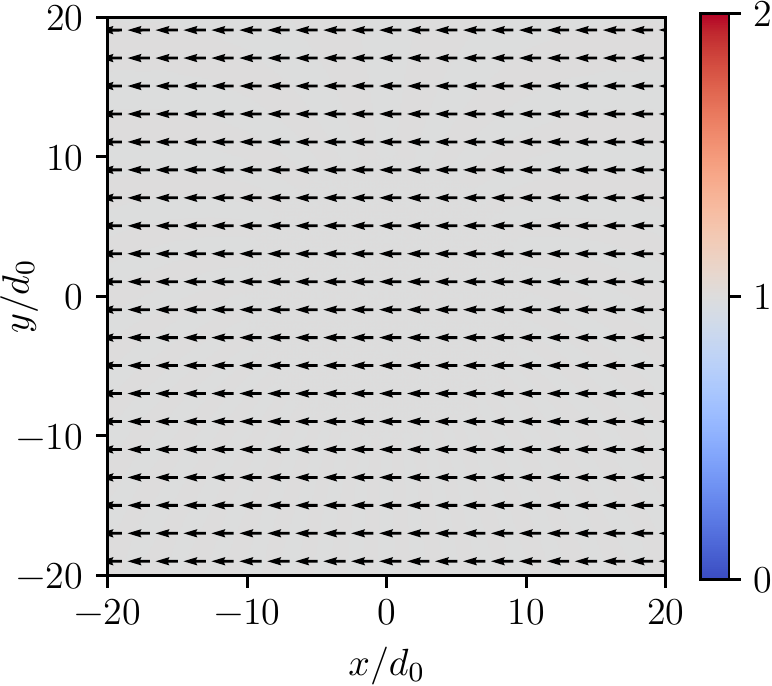}
			\caption{$s=-1$, $\alpha = 0$}
			\vspace*{0pt}
			\label{figIso3b}
		\end{subfigure}
	\end{figure}
	
	\begin{figure}[!h]
		\ContinuedFloat
		\begin{subfigure}{0.49\linewidth}
			\centering
			\includegraphics[scale=0.833]{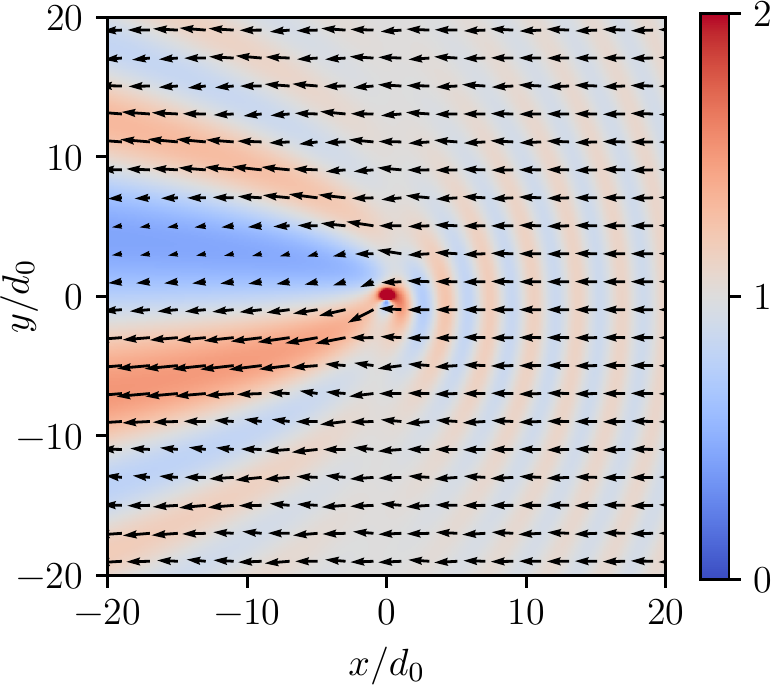}
			\caption{$s=1$, $\alpha = 0.2$}
			\vspace*{5pt}
			\label{figIso3c}
		\end{subfigure}
		\begin{subfigure}{0.49\linewidth}
			\centering
			\includegraphics[scale=0.833]{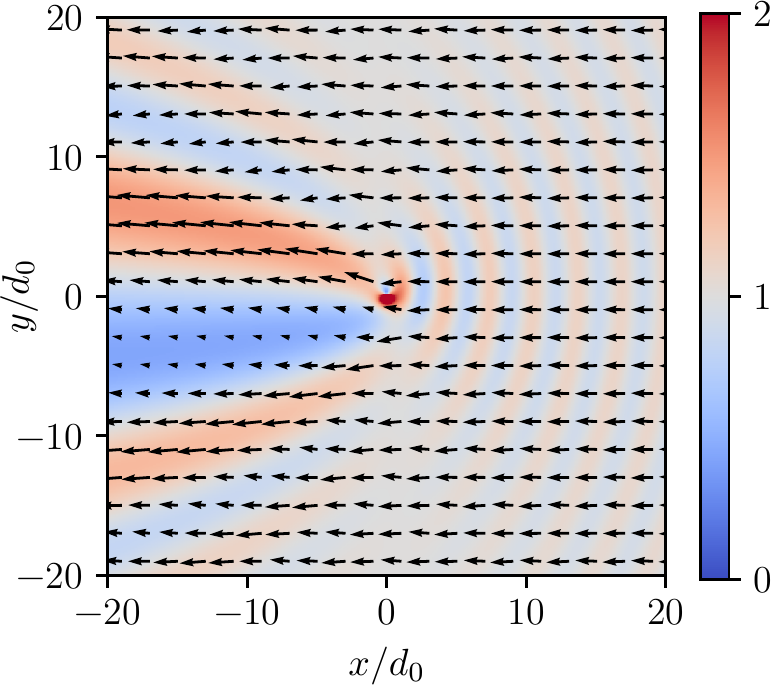}
			\caption{$s=-1$, $\alpha = 0.2$}
			\vspace*{5pt}
			\label{figIso3d}
		\end{subfigure}
		\begin{subfigure}{0.49\linewidth}
			\centering
			\includegraphics[scale=0.833]{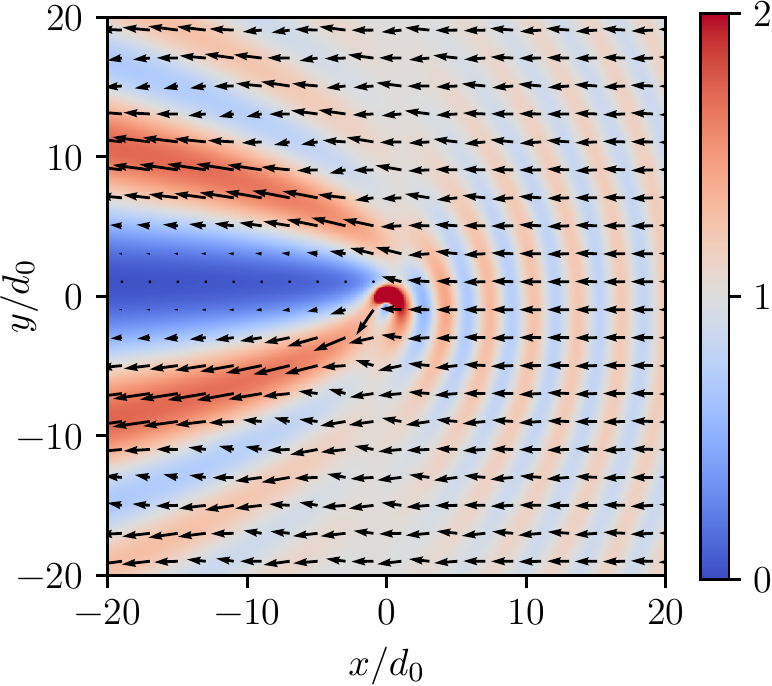}
			\caption{$s=1$, $\alpha = 0.5$}
			\vspace*{5pt}
			\label{figIso3e}
		\end{subfigure}
		\begin{subfigure}{0.49\linewidth}
			\centering
			\includegraphics[scale=0.833]{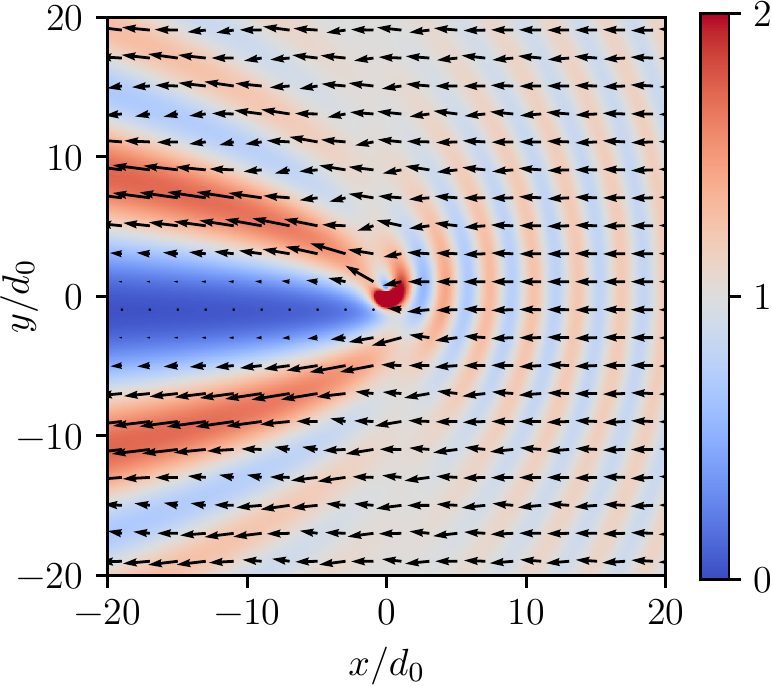}
			\caption{$s=-1$, $\alpha = 0.5$}
			\vspace*{5pt}
			\label{figIso3f}
		\end{subfigure}
		\begin{subfigure}{0.49\linewidth}
			\centering
			\includegraphics[scale=0.833]{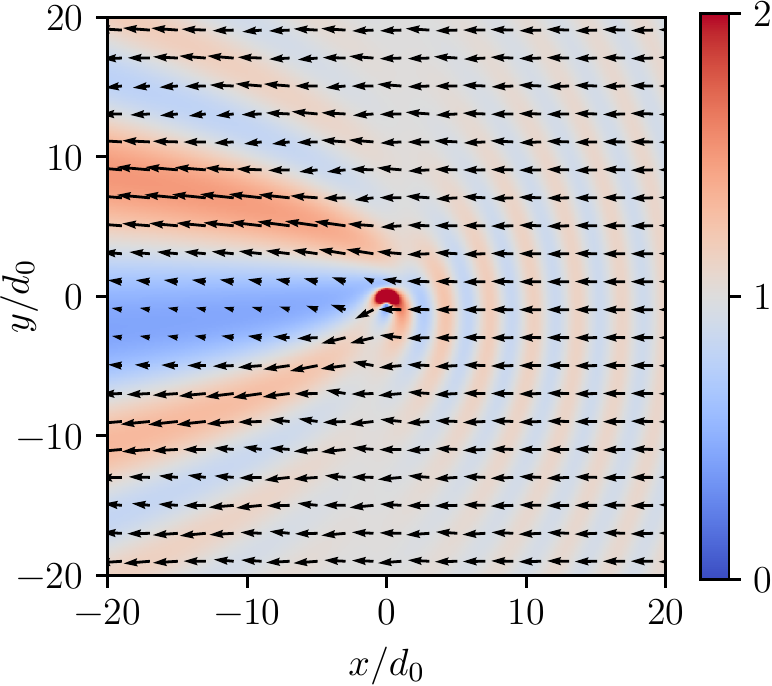}
			\caption{$s=1$, $\alpha = 0.8$}
			\vspace*{5pt}
			\label{figIso3g}
		\end{subfigure}
		\begin{subfigure}{0.49\linewidth}
			\centering
			\includegraphics[scale=0.833]{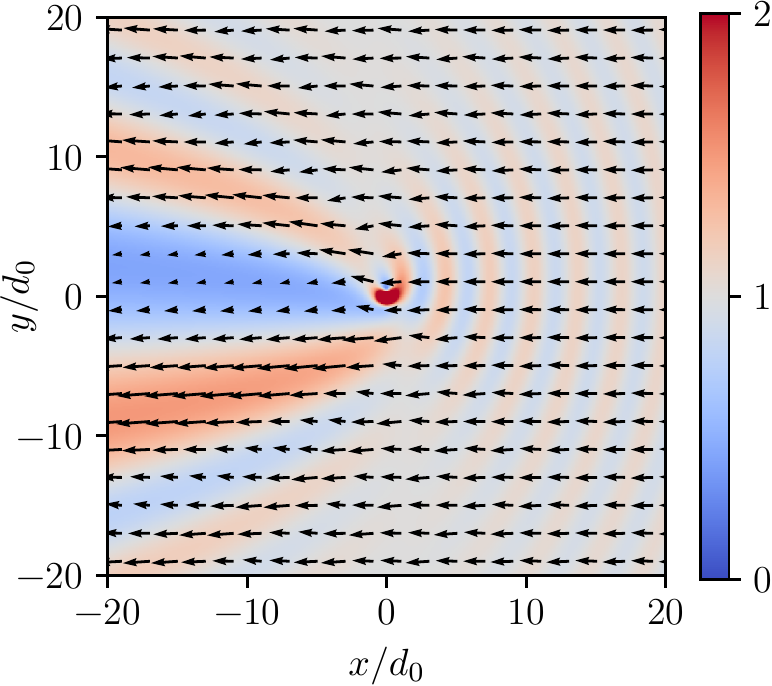}
			\caption{$s=-1$, $\alpha = 0.8$}
			\vspace*{5pt}
			\label{figIso3h}
		\end{subfigure}
		\caption{Scattering states corresponding to the Aharonov--Bohm effect in bilayer graphene. The probability density $\varrho$ (represented by the colors) and current density $\boldsymbol{j}$ (represented by the arrows) are computed for $kd_0 = 1$ (where $d_0$ is a natural length unit) and different values of the parameters $s$ and $\alpha$.}
		\label{figIso3}
	\end{figure}
	
	
	\subsection{Electron Gas with Rashba Effect}
	\label{graphene:supp_sec}
	
	The fourth example to be discussed is the \emph{two-dimensional electron gas subject to the Rashba effect} which appears in semiconducting heterostructures where the spin-orbit coupling is sufficiently large. Additionally, to the appearance of the Rashba effect, it is required that a crystal has a single high-symmetry axis \cite{Rashba_cikk_1960}. This is naturally true for heterojunctions (e.g., GaAs-AlGaAs) where the aforementioned direction is the normal of the interface \cite{Yu_A_Bychkov_1984,Fabian_RevModPhys.76.323,Winkler:684956}. The spin-orbit interaction in these systems can be well described by a Hamiltonian term linear in both the momentum and the spin operators. To the best of our knowledge, the Aharonov--Bohm effect in this system has not been investigated before. In the following, we aim to do so using our newly developed methods.
	
	%\subsubsection{Hamiltonian Operator}
	%\label{subsec351}
	
	The Hilbert space corresponding to the two-dimensional electron gas with Rashba effect is $\mathcal{H} = L^2(\mathbb{R}^2,\mathbb{C})\otimes\mathbb{C}^2$, that is, there is a two-state inner degree of freedom ($D=2$) corresponding to the spin of the electron. The Hamiltonian operator $\hat{H}: \mathcal{D}_H \to \mathcal{H}$ is given as a quadratic polynomial of the momentum operators:
	\begin{equation}
		\hat{H} = \frac{1}{2M} \left(\hat{p}_x^2 + \hat{p}_y^2\right)\otimes\hat{I} + v \left(\hat{p}_y\otimes\hat{\sigma}_x - \hat{p}_x\otimes\hat{\sigma}_y\right) ,
		\label{eqIso25}
	\end{equation} where $M$ and $v$ are an effective mass and an effective velocity parameter, respectively, and $\hat{\sigma}_x$, $\hat{\sigma}_y$ and $\hat{\sigma}_z$ are the Pauli operators defined in Eq.\ \eqref{eqIso9}. 
	
	%\subsubsection{Band Structure and its Properties}
	%\label{subsec352}
	
	The band structure corresponding to the Hamiltonian in Eq.\ \eqref{eqIso25} consists of two bands with $s\in\{-1,1\}$ which are given in polar coordinates as:
	\begin{equation}
		E_s(k,\vartheta) = \frac{\hbar^2 k^2}{2M} + sv\hbar k .
		\label{eqIso26}
	\end{equation} As expected, the isotropy of the system is manifested in the shape of the band structure: the constant energy curves are circles for all values of the energy. The momentum space eigenvectors need to be chosen such that one of its components is independent of $\vartheta$. We can choose this to be the upper component:
	\begin{equation}
		\mathbf{u}_s(k,\vartheta) = \frac{1}{\sqrt2} \begin{pmatrix} 1 \\ -\iu s \euler^{\iu\vartheta} \end{pmatrix} .
		\label{eqIso27}
	\end{equation}
	
	%\begin{figure}[hbt]
	%\centering
	%\vspace*{-20pt}
	%\includegraphics[scale=0.833]{Rashba_Bands1.pdf}\hspace{10pt}
	%\includegraphics[scale=0.833]{Rashba_Bands2.pdf}
	%\caption{Surface plot (on the left) and contour plot (on the right) corresponding to the band structure of the two-dimensional electron gas with Rashba effect in Equation \eqref{eqIso48}. Natural length and energy units $d_0$ and $E_0$ were used to make the scales dimensionless. The parameters are chosen such that $\hbar v = E_0d_0$.}
	%\label{figIso10}
	%\end{figure}
	
	The group velocity vector field is easily determined from Eq.\ \eqref{eqIso25} by taking its gradient with respect to $\hbar\boldsymbol{k}$. The results are the following:
	\begin{subequations}
		\begin{align}
			v_{s,k}(k,\vartheta) &= \frac{\hbar k}{M} + sv , 
			\label{eqIso28a} \\
			v_{s,\vartheta}(k,\vartheta) &= 0 . 
			\label{eqIso28b}
		\end{align} 
	\end{subequations} It is clearly seen that the radial group velocity is everywhere positive for the band with $s=1$, we can call it electron-like. However, the sign of the group velocity varies for $s=-1$. More concretely, there is a critical wave number
	\begin{equation}
		k_\mathrm{c} = \frac{Mv}{\hbar}
		\label{eqIso29}
	\end{equation} above (below) which $v_{s,k}$ is positive (negative). Based on this we can call the band with $s=-1$ \emph{mixed}.
	
	%\subsubsection{Probability Current}
	
	A further important quantity is the probability density of the electron position corresponding to an arbitrary state $\boldsymbol{\Psi} = \left(\Psi_1,\Psi_2\right) \in \mathcal{H}$. This can be written as a special case of Eq.\ \eqref{eqCross2} for this two-band system:
	\begin{equation}
		\varrho = \Psi_1^* \Psi_1 + \Psi_2^* \Psi_2 .
		\label{eqIso30}
	\end{equation} The probability current density on the other hand depends on the Hamiltonian in Eq.\ \eqref{eqIso25} as well. Applying the results of Eqs.\ \eqref{eqCross6a} and \eqref{eqCross6b} we find:
	\begin{subequations}
		\begin{align}
			j_x &= \frac{1}{M}~\mathrm{Re}\left[\Psi_1^* \big(\hat{\Pi}_x \Psi_1\big) + \Psi_2^*\big(\hat{\Pi}_x \Psi_2\big)\right] + 2v~\mathrm{Im}\left(\Psi_1\Psi_2^*\right)  , 
			\label{eqIso31a} \\
			j_y &= \frac{1}{M}~\mathrm{Re}\left[\Psi_1^* \big(\hat{\Pi}_y \Psi_1\big) + \Psi_2^*\big(\hat{\Pi}_y \Psi_2\big)\right] + 2v~\mathrm{Re}\left(\Psi_1\Psi_2^*\right) . 
			\label{eqIso31b}
		\end{align}
	\end{subequations}
	
	%\subsubsection{Scattering States}
	
	With all the ingredients collected, now Eq.~(5) of the main text can be applied to calculate the scattering states. The integral representation of the Bessel functions can again be used \cite{Grads:book}, the final result for the electron-like band with $s=1$ is
	\begin{equation}
		\boldsymbol{\Psi}^{(+)}_{1,\boldsymbol{k}}(r,\varphi) = \sum_{m=-\infty}^\infty \frac{(-\iu)^{|m+\alpha|} \euler^{\iu m (\varphi - \vartheta + \pi)}}{\sqrt2} \begin{pmatrix} J_{|m+\alpha|}(k r) \\ \epsilon(m + \alpha) J_{|m+\alpha| + \epsilon(m+\alpha)}(k r) \euler^{\iu\varphi} \end{pmatrix} ,
		\label{eqIso32}
	\end{equation} for the mixed band with $s=-1$ and $k < k_\mathrm{c}$ is
	\begin{equation}
		\boldsymbol{\Psi}^{(+)}_{-1,\boldsymbol{k}}(r,\varphi) = \sum_{m=-\infty}^\infty \frac{\iu^{|m+\alpha|} \euler^{\iu m (\varphi - \vartheta + \pi)}}{\sqrt2} \begin{pmatrix} J_{|m+\alpha|}(k r) \\ -\epsilon(m + \alpha) J_{|m+\alpha| + \epsilon(m+\alpha)}(k r) \euler^{\iu\varphi} \end{pmatrix} ,
		\label{eqIso33}
	\end{equation} whereas for the mixed band with $s=-1$ and $k > k_\mathrm{c}$ is
	\begin{equation}
		\boldsymbol{\Psi}^{(+)}_{-1,\boldsymbol{k}}(r,\varphi) = \sum_{m=-\infty}^\infty \frac{(-\iu)^{|m+\alpha|} \euler^{\iu m (\varphi - \vartheta + \pi)}}{\sqrt2} \begin{pmatrix} J_{|m+\alpha|}(k r) \\ -\epsilon(m + \alpha) J_{|m+\alpha| + \epsilon(m+\alpha)}(k r) \euler^{\iu\varphi} \end{pmatrix} .
		\label{eqIso34}
	\end{equation} To the best of our knowledge, these results cannot be found in the literature.
	
	The probability density and current density corresponding to these scattering states can again be numerically evaluated utilizing Eqs.\ \eqref{eqIso30}, \eqref{eqIso31a} and \eqref{eqIso31b}, the results are shown in Fig.\ \ref{figIso4}. These are quite similar to the case of monolayer graphene discussed before, there is only one difference worth mentioning. In the case of the mixed band with $s=-1$, there are two significantly different regimes separated in Eqs.\ \eqref{eqIso33} and \eqref{eqIso34}. From these, Fig.\ \ref{figIso4} shows only the second one where $k>k_\mathrm{c}$. In this case, the probability density is perfectly identical to that of the $s=1$ band as can be seen by the comparison of Fig.\ \ref{figIso4c} and \ref{figIso4d} for instance. However, the current densities are noticeably different. The $k<k_\mathrm{c}$ case is not depicted in the figures as it is very similar to the hole-like band of monolayer graphene. That is, both the probability density and the current density becomes noticeably different from those of the electron-like upper band.
	
	\begin{figure}[hbt]
		\begin{subfigure}{0.49\linewidth}
			\centering
			\includegraphics[scale=0.833]{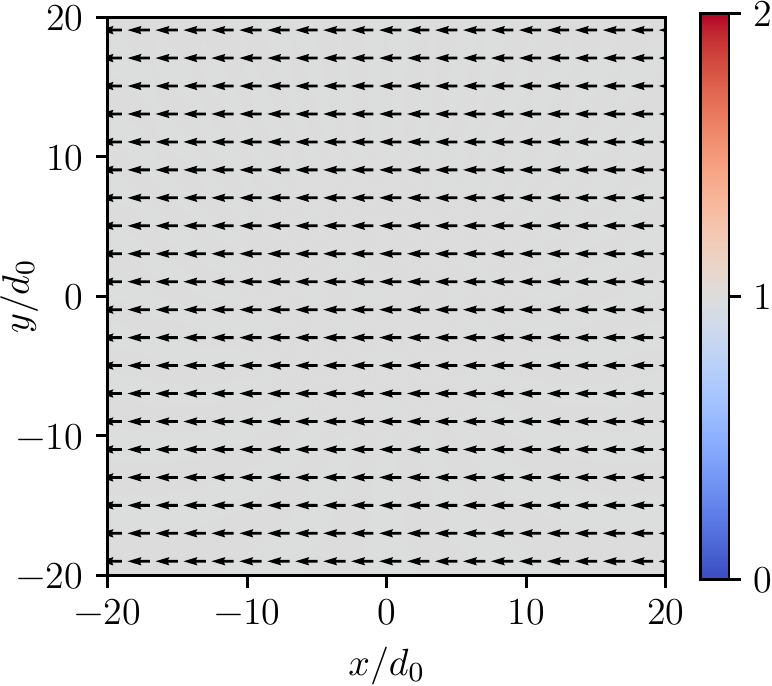}
			\caption{$s=1$, $\alpha = 0$}
			\vspace*{5pt}
			\label{figIso4a}
		\end{subfigure}
		\begin{subfigure}{0.49\linewidth}
			\centering
			\includegraphics[scale=0.833]{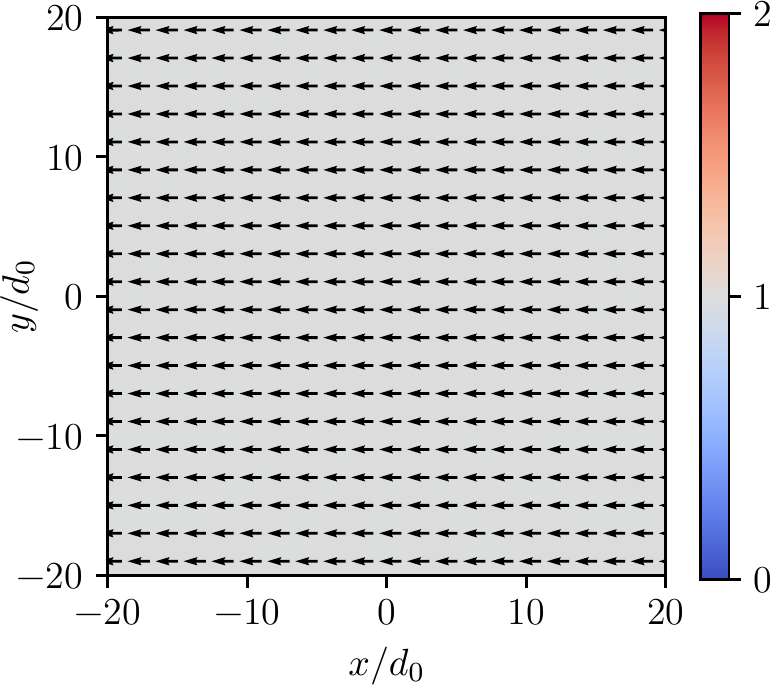}
			\caption{$s=-1$, $\alpha = 0$}
			\vspace*{5pt}
			\label{figIso4b}
		\end{subfigure}
		\begin{subfigure}{0.49\linewidth}
			\centering
			\includegraphics[scale=0.833]{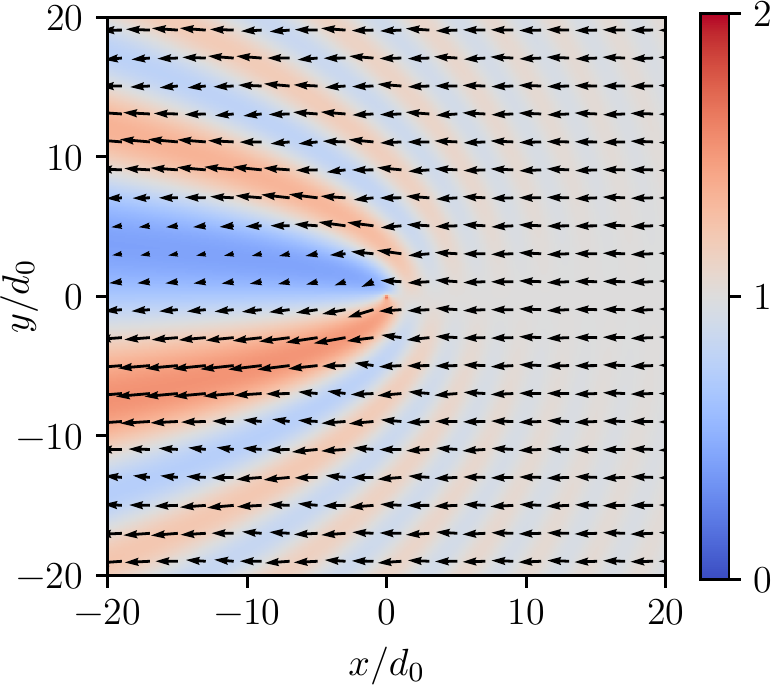}
			\caption{$s=1$, $\alpha = 0.2$}
			\vspace*{0pt}
			\label{figIso4c}
		\end{subfigure}
		\begin{subfigure}{0.49\linewidth}
			\centering
			\includegraphics[scale=0.833]{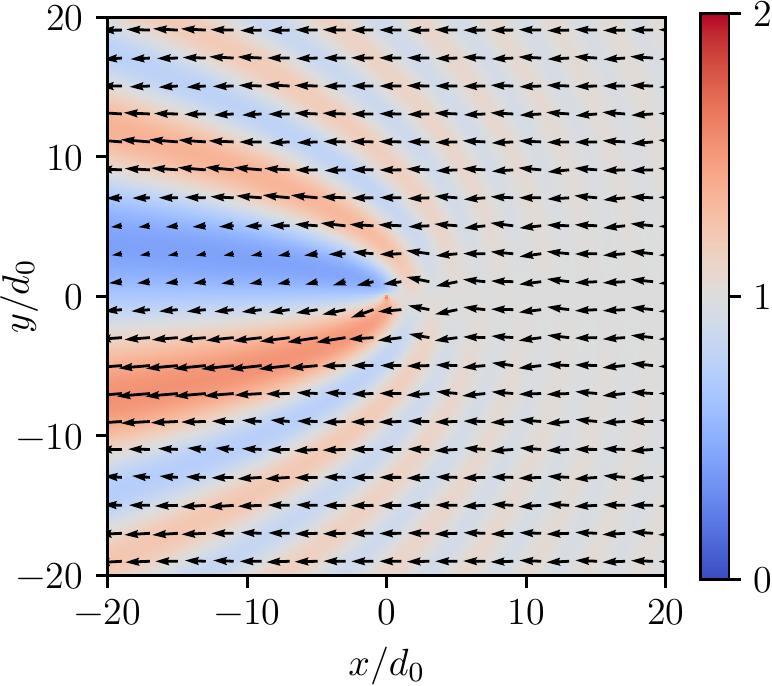}
			\caption{$s=-1$, $\alpha = 0.2$}
			\vspace*{0pt}
			\label{figIso4d}
		\end{subfigure}
	\end{figure}
	
	\begin{figure}[!h]
		\ContinuedFloat
		\begin{subfigure}{0.49\linewidth}
			\centering
			\includegraphics[scale=0.833]{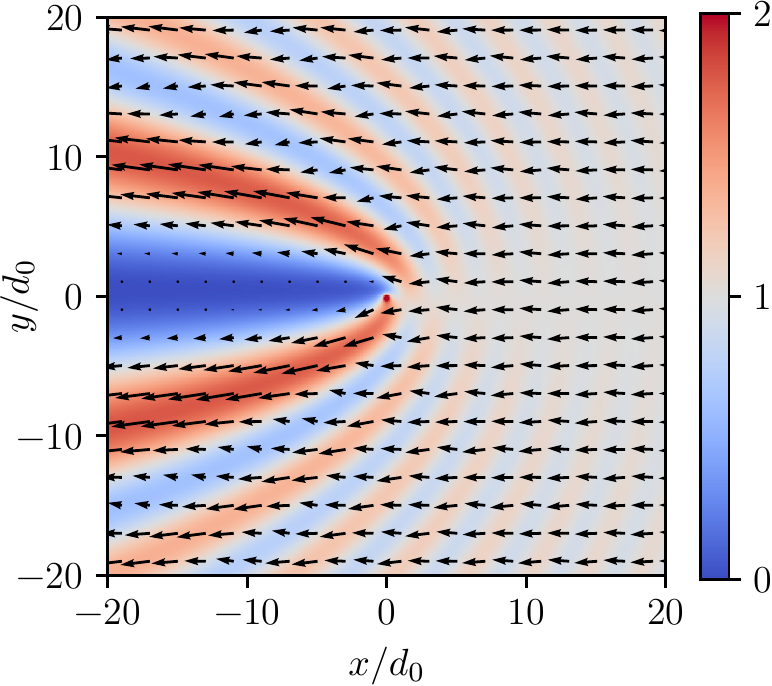}
			\caption{$s=1$, $\alpha = 0.5$}
			\vspace*{5pt}
			\label{figIso4e}
		\end{subfigure}
		\begin{subfigure}{0.49\linewidth}
			\centering
			\includegraphics[scale=0.833]{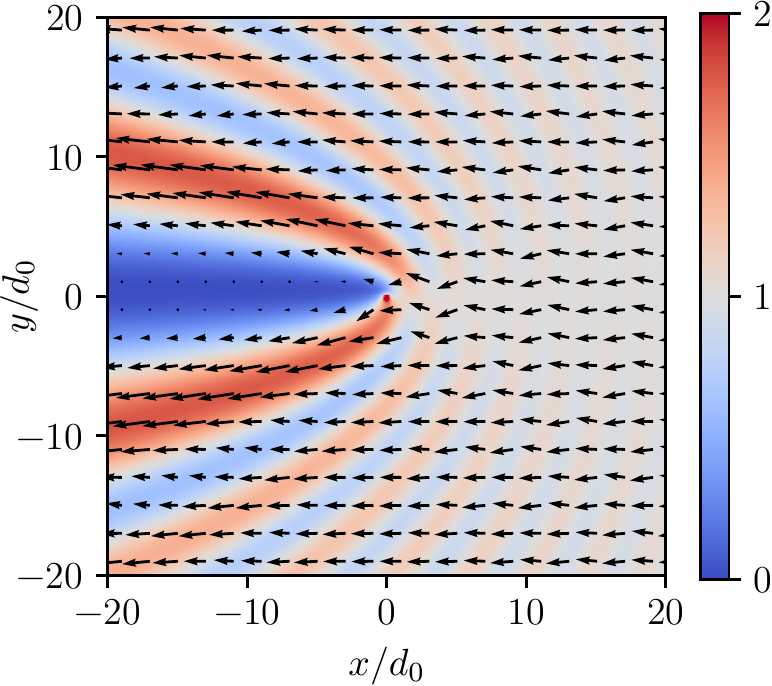}
			\caption{$s=-1$, $\alpha = 0.5$}
			\vspace*{5pt}
			\label{figIso4f}
		\end{subfigure}
		\begin{subfigure}{0.49\linewidth}
			\centering
			\includegraphics[scale=0.833]{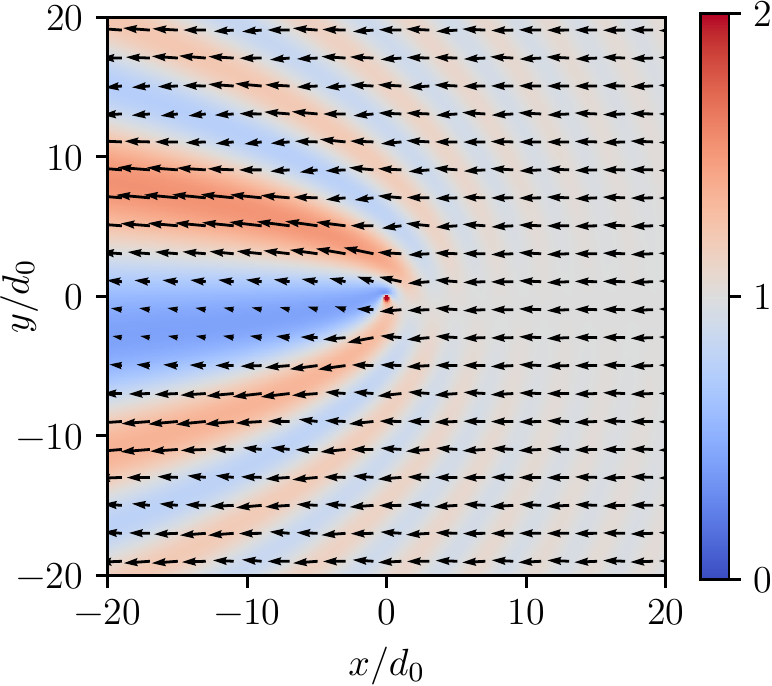}
			\caption{$s=1$, $\alpha = 0.8$}
			\vspace*{5pt}
			\label{figIso4g}
		\end{subfigure}
		\begin{subfigure}{0.49\linewidth}
			\centering
			\includegraphics[scale=0.833]{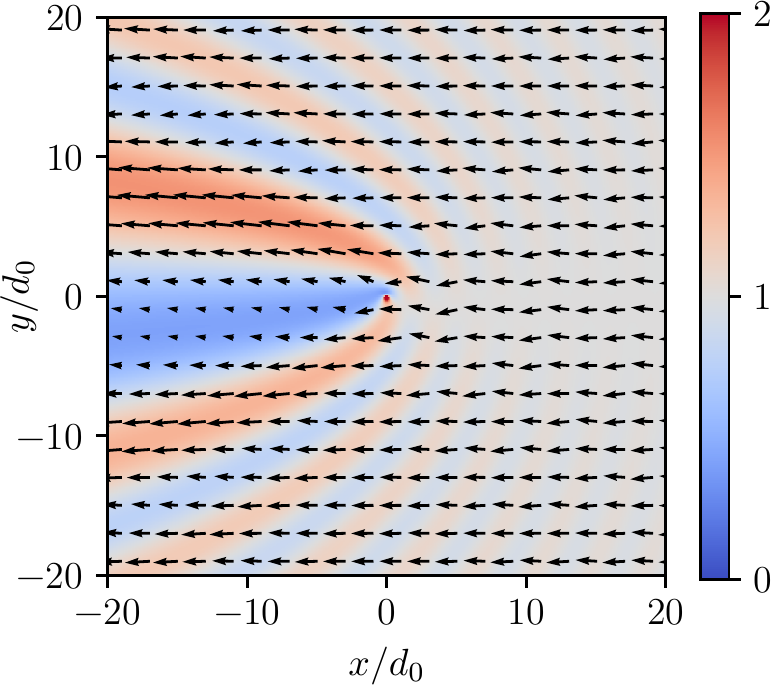}
			\caption{$s=-1$, $\alpha = 0.8$}
			\vspace*{5pt}
			\label{figIso4h}
		\end{subfigure}
		\caption{Scattering states corresponding to the Aharonov--Bohm effect in the Rashba system. The probability density $\varrho$ (represented by the colors) and current density $\boldsymbol{j}$ (represented by the arrows) are computed for $kd_0 = 1$ (where $d_0$ is a natural length unit) and different values of the parameters $s$ and $\alpha$.}
		\label{figIso4}
	\end{figure}
	
	\subsection{Pseudospin-1 System}
	\label{dice:supp_sec}
	
	The fifth example to be discussed is the \emph{Lieb lattice}, that is, a two-dimensional face-centered-square lattice \cite{PhysRevB.84.115136,PhysRevB.81.041410,PhysRevA.80.063603,PhysRevB.84.195422}. In such a system, the band structure contains a single Dirac point in the Brillouin zone where two conic and a flat band touch. Similarly to graphene, a low energy effective model can be applied in which the dynamics of electrons are analogous to that of massless spin-$1$ relativistic particles. The same phenomenon can be observed in other materials such as the \emph{dice lattice} where two pseudospin-$1$ Dirac points appear in the Brillouin zone. To the best of our knowledge, the Aharonov--Bohm effect in this system has not been investigated before. In the following, we aim to do so using our newly developed methods.
	
	%\subsubsection{Hamiltonian Operator}
	%\label{subsec361}
	
	The Hilbert space corresponding to the Lieb lattice is $\mathcal{H} = L^2(\mathbb{R}^2,\mathbb{C})\otimes\mathbb{C}^3$, that is, there is a three-state inner degree of freedom ($D=3$) corresponding to the three sublattices of the crystal. The Hamiltonian operator $\hat{H}: \mathcal{D}_H \to \mathcal{H}$ is given as a linear polynomial of the momentum operators:
	\begin{equation}
		\hat{H} = v \big(\hat{p}_x\otimes\hat{\tau}_x + \hat{p}_y\otimes\hat{\tau}_y\big) ,
		\label{eqIso35}
	\end{equation} where $v$ is an effective velocity parameter and 
	\begin{equation}
		\hat{\tau}_x = \frac{1}{\sqrt2} \begin{pmatrix}
			~0~ & ~1~ & ~0~ \\ ~1~ & ~0~ & ~1~ \\ ~0~ & ~1~ & ~0~
		\end{pmatrix} ,~~~~~ \hat{\tau}_y = \frac{\iu}{\sqrt2} \begin{pmatrix}
			~0~ & -1~ & ~0~ \\ ~1~ & ~0~ & -1~ \\ ~0~ & ~1~ & ~0~
		\end{pmatrix} ,~~~~~ \hat{\tau}_z = \begin{pmatrix}
			~1~ & ~0~ & ~0~ \\ ~0~ & ~0~ & ~0~ \\ ~0~ & ~0~ & -1~
		\end{pmatrix} .
		\label{eqIso36}
	\end{equation} are the \emph{spin-1 operators} corresponding to the three-dimensional representation of $\mathfrak{so}(3)$ given as matrices. 
	
	%\subsubsection{Band Structure and its Properties}
	%\label{subsec362}
	
	The band structure corresponding to the Hamiltonian in Eq.\ \eqref{eqIso35} consists of three bands with $s\in\{-1,0,1\}$ which are given in polar coordinates as:
	\begin{equation}
		E_s(k,\vartheta) = s v \hbar k .
		\label{eqIso37}
	\end{equation} As expected, the isotropy of the system is manifested in the shape of the band structure: the constant energy curves are circles for all values of the energy. The momentum space eigenvectors need to be chosen such that one of its components is independent of $\vartheta$. We can choose this to be the middle component:
	\begin{subequations}
		\begin{alignat}{2}
			\mathbf{u}_s(k,\vartheta) &= \frac{1}{2} \begin{pmatrix} \euler^{-\iu\vartheta} \\ \sqrt2 s \\ \euler^{\iu\vartheta} \end{pmatrix} , &&\mathrm{if}~s = \pm 1, \label{eqIso36a} \\
			\mathbf{u}_s(k,\vartheta) &= \frac{1}{\sqrt2} \begin{pmatrix} \euler^{-\iu\vartheta} \\ 0 \\ -\euler^{\iu\vartheta} \end{pmatrix} ,~~~ &&\mathrm{if}~s = 0. \label{eqIso36b}
		\end{alignat}
	\end{subequations}
	
	%\begin{figure}[hbt]
	%\centering
	%\vspace*{-20pt}
	%\includegraphics[scale=0.833]{Pseudospin_Bands1.pdf}\hspace{10pt}
	%\includegraphics[scale=0.833]{Pseudospin_Bands2.pdf}
	%\caption{Surface plot (on the left) and contour plot (on the right) corresponding to the band structure of the Lieb lattice in Equation \eqref{eqIso63}. Natural length and energy units $d_0$ and $E_0$ were used to make the scales dimensionless.}
	%\label{figIso12}
	%\end{figure}
	
	\begin{figure}[!h]
		\begin{subfigure}{0.49\linewidth}
			\centering
			\includegraphics[scale=0.833]{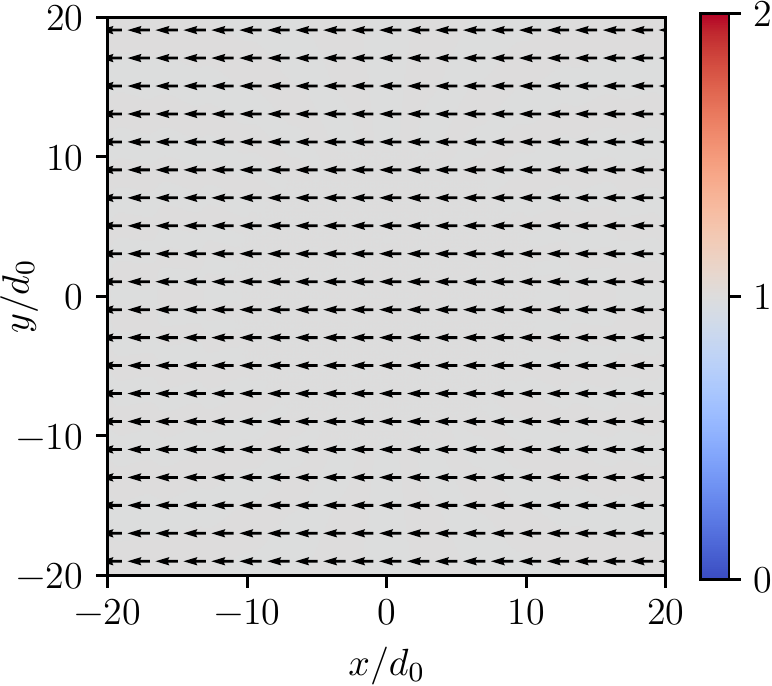}
			\caption{$s=1$, $\alpha = 0$}
			\vspace*{5pt}
			\label{figIso5a}
		\end{subfigure}
		\begin{subfigure}{0.49\linewidth}
			\centering
			\includegraphics[scale=0.833]{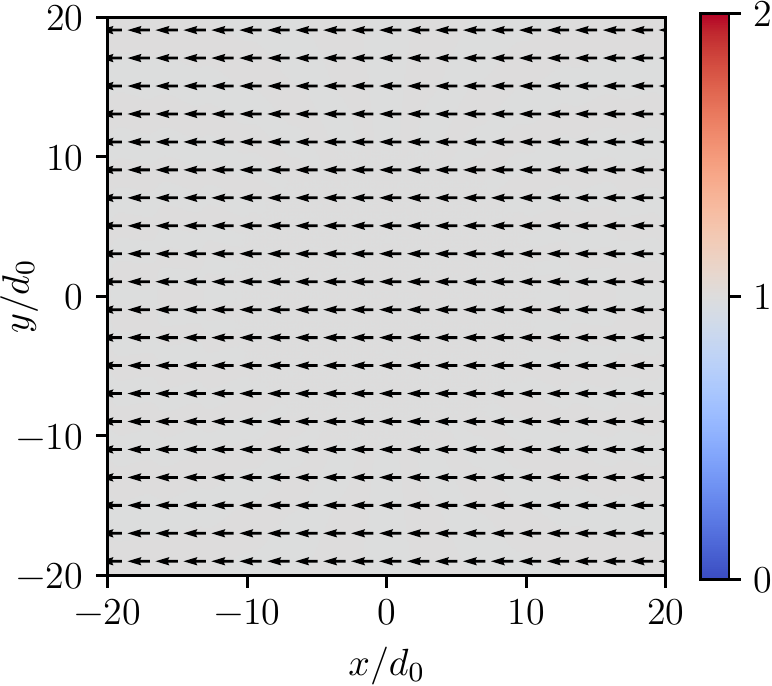}
			\caption{$s=-1$, $\alpha = 0$}
			\vspace*{5pt}
			\label{figIso5b}
		\end{subfigure}
		\begin{subfigure}{0.49\linewidth}
			\centering
			\includegraphics[scale=0.833]{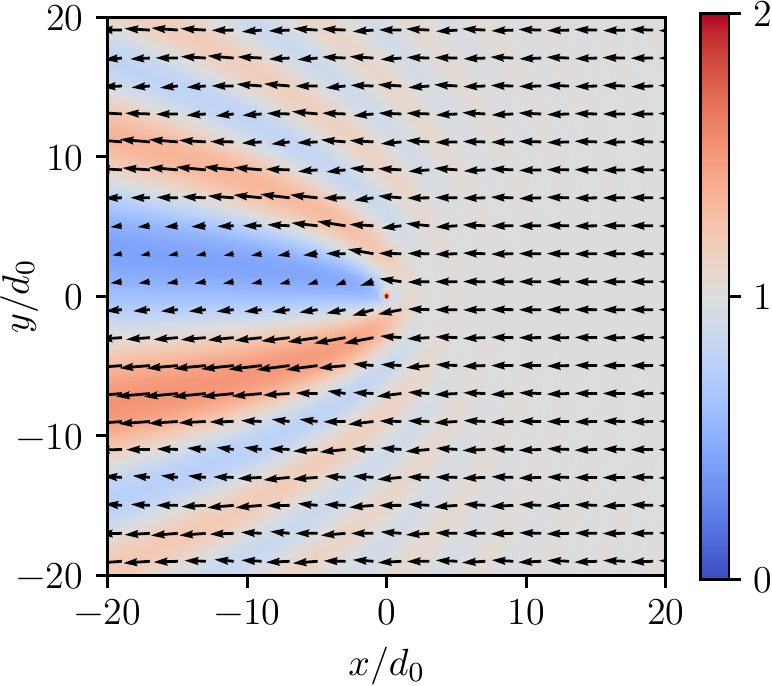}
			\caption{$s=1$, $\alpha = 0.2$}
			\vspace*{5pt}
			\label{figIso5c}
		\end{subfigure}
		\begin{subfigure}{0.49\linewidth}
			\centering
			\includegraphics[scale=0.833]{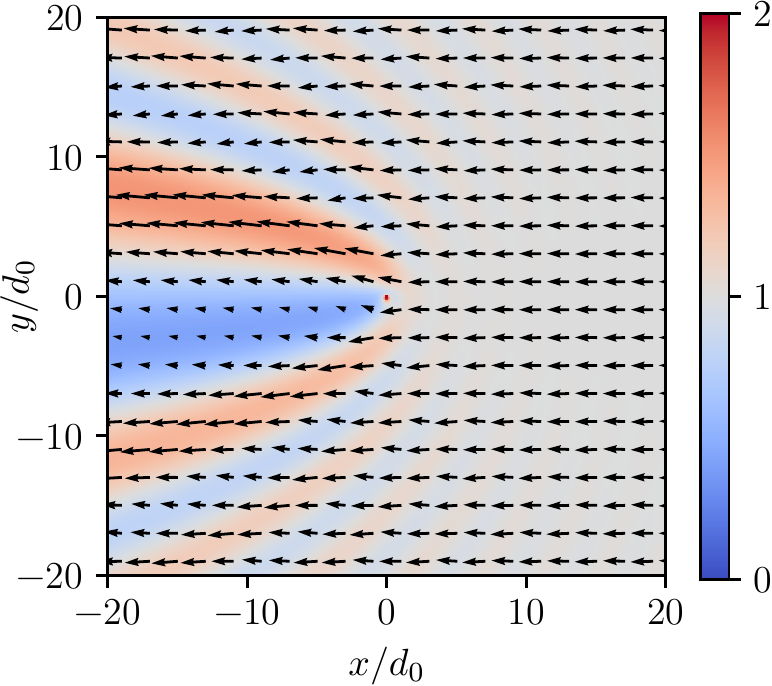}
			\caption{$s=-1$, $\alpha = 0.2$}
			\vspace*{5pt}
			\label{figIso5d}
		\end{subfigure}
	\end{figure}
	
	The group velocity vector field is easily determined from Eq.\ \eqref{eqIso37} by taking its gradient with respect to $\hbar\boldsymbol{k}$. The results are the following:
	\begin{subequations}
		\begin{align}
			v_{s,k}(k,\vartheta) &= sv , 
			\label{eqIso37a} \\
			v_{s,\vartheta}(k,\vartheta) &= 0 . 
			\label{eqIso37b}
		\end{align} 
	\end{subequations} It is clearly seen that the radial group velocity is either everywhere positive, everywhere zero, or everywhere negative depending on the band index $s$. This implies that the band with $s=1$ is electron-like whereas the band with $s=-1$ is hole-like. The band with $s=0$ is a non-dispersive so-called \emph{flat band}, plane waves corresponding to this band have a constant zero current density, in other words, they are not propagating states. Consequently, it is meaningless to investigate the scattering problem in this case.
	
	\begin{figure}[!h]
		\ContinuedFloat
		\begin{subfigure}{0.49\linewidth}
			\centering
			\includegraphics[scale=0.833]{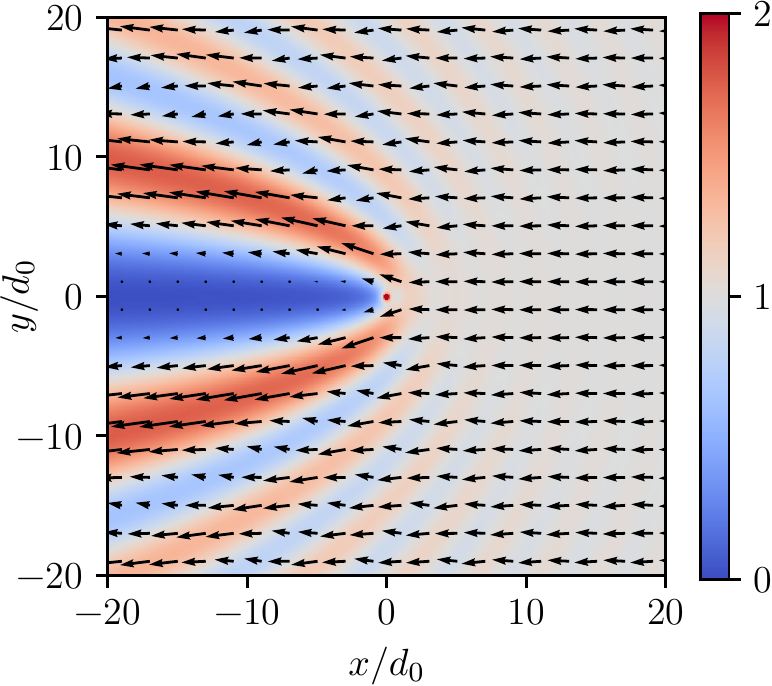}
			\caption{$s=1$, $\alpha = 0.5$}
			\vspace*{5pt}
			\label{figIso5e}
		\end{subfigure}
		\begin{subfigure}{0.49\linewidth}
			\centering
			\includegraphics[scale=0.833]{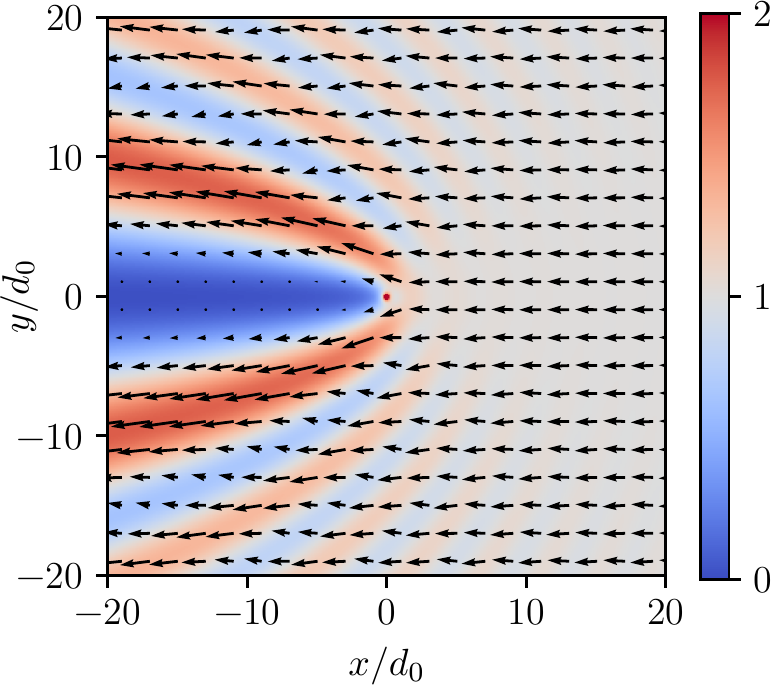}
			\caption{$s=-1$, $\alpha = 0.5$}
			\vspace*{5pt}
			\label{figIso5f}
		\end{subfigure}
		\begin{subfigure}{0.49\linewidth}
			\centering
			\includegraphics[scale=0.833]{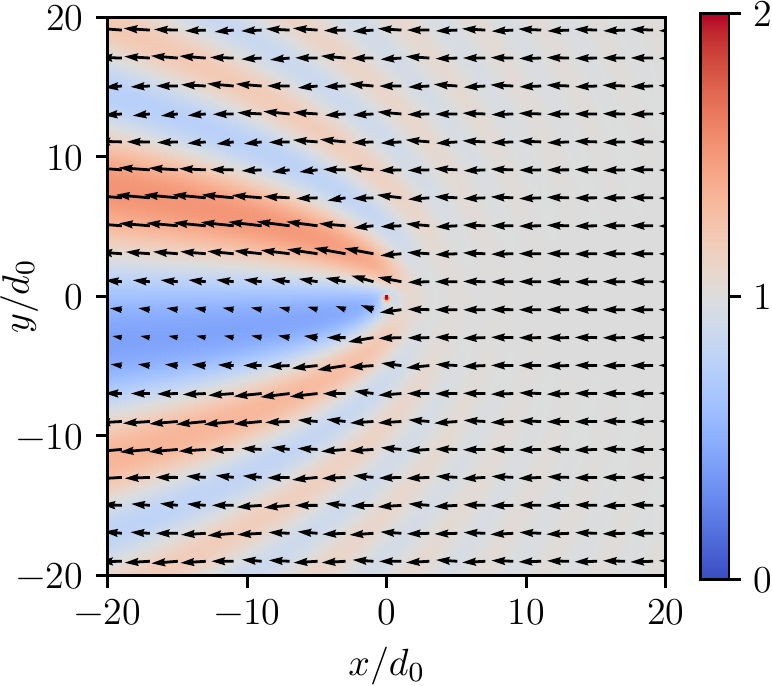}
			\caption{$s=1$, $\alpha = 0.8$}
			\vspace*{5pt}
			\label{figIso5g}
		\end{subfigure}
		\begin{subfigure}{0.49\linewidth}
			\centering
			\includegraphics[scale=0.833]{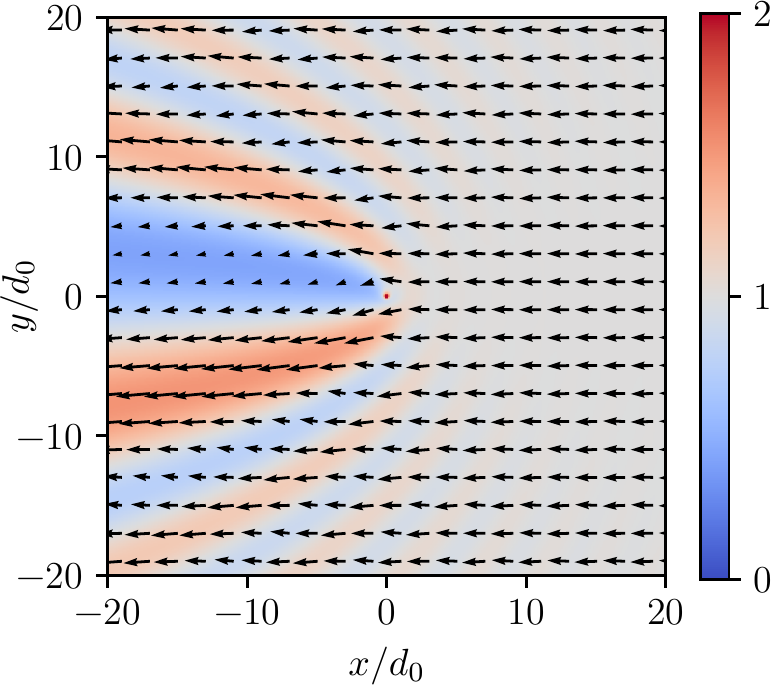}
			\caption{$s=-1$, $\alpha = 0.8$}
			\vspace*{5pt}
			\label{figIso5h}
		\end{subfigure}
		\caption{Scattering states corresponding to the Aharonov--Bohm effect in the Lieb lattice. The probability density $\varrho$ (represented by the colors) and current density $\boldsymbol{j}$ (represented by the arrows) are computed for $kd_0 = 1$ (where $d_0$ is a natural length unit) and different values of the parameters $s$ and $\alpha$.}
		\label{figIso5}
	\end{figure}
	
	%\subsubsection{Probability Current}
	
	A further important quantity is the probability density of the electron position corresponding to an arbitrary state $\boldsymbol{\Psi} = \left(\Psi_1,\Psi_2,\Psi_3\right) \in \mathcal{H}$. This can be written as a special case of Eq.\ \eqref{eqCross2} for this three-band system:
	\begin{equation}
		\varrho = \Psi_1^* \Psi_1 + \Psi_2^* \Psi_2 + \Psi_3^* \Psi_3 .
		\label{eqIso38}
	\end{equation} The probability current density on the other hand depends on the Hamiltonian in Eq.\ \eqref{eqIso35} as well. Applying the results of Eqs.\ \eqref{eqCross6a} and \eqref{eqCross6b} we find:
	\begin{subequations}
		\begin{align}
			j_x &= \sqrt2 v~\mathrm{Re}\left(\Psi_1^*\Psi_2 + \Psi_2^*\Psi_3\right), 
			\label{eqIso39a} \\
			j_y &= \sqrt2 v~\mathrm{Im}\left(\Psi_1^*\Psi_2 + \Psi_2^*\Psi_3\right). 
			\label{eqIso39b}
		\end{align}
	\end{subequations}
	
	%\subsubsection{Scattering States}
	
	With all the ingredients collected, now Eq.~(5) of the main text can be applied to calculate the scattering states. The integral representation of the Bessel functions can again be used \cite{Grads:book}, the final result for the electron-like band with $s=1$ is
	\begin{equation}
		\boldsymbol{\Psi}^{(+)}_{1,\boldsymbol{k}}(r,\varphi) = \sum_{m=-\infty}^\infty \frac{(-\iu)^{|m+\alpha|} \euler^{\iu m (\varphi - \vartheta + \pi)}}{2 \iu} \begin{pmatrix} \epsilon(m + \alpha) J_{|m+\alpha| - \epsilon(m+\alpha)}(k r) \euler^{-\iu\varphi} \\ \sqrt2 \iu ~ J_{|m+\alpha|}(k r) \\ \epsilon(m + \alpha) J_{|m+\alpha| + \epsilon(m+\alpha)}(k r) \euler^{\iu\varphi} \end{pmatrix} ,
		\label{eqIso40}
	\end{equation} whereas for the hole-like band with $s=-1$ is
	\begin{equation}
		\boldsymbol{\Psi}^{(+)}_{-1,\boldsymbol{k}}(r,\varphi) = \sum_{m=-\infty}^\infty \frac{\iu^{|m+\alpha|} \euler^{\iu m (\varphi - \vartheta + \pi)}}{2 \iu} \begin{pmatrix} \epsilon(m + \alpha) J_{|m+\alpha| - \epsilon(m+\alpha)}(k r) \euler^{-\iu\varphi} \\ -\sqrt2 \iu ~ J_{|m+\alpha|}(k r) \\ \epsilon(m + \alpha) J_{|m+\alpha| + \epsilon(m+\alpha)}(k r) \euler^{\iu\varphi} \end{pmatrix} .
		\label{eqIso41}
	\end{equation} To the best of our knowledge, these results cannot be found in the literature.
	
	The probability density and current density corresponding to these scattering states can again be numerically evaluated utilizing Eqs.\ \eqref{eqIso38}, \eqref{eqIso39a} and \eqref{eqIso39b}, the results are shown in Fig.\ \ref{figIso5}. These are quite similar to the case of monolayer graphene discussed before.
	
	
	
	%apsrev4-2.bst 2019-01-14 (MD) hand-edited version of apsrev4-1.bst
	%Control: key (0)
	%Control: author (8) initials jnrlst
	%Control: editor formatted (1) identically to author
	%Control: production of article title (0) allowed
	%Control: page (0) single
	%Control: year (1) truncated
	%Control: production of eprint (0) enabled
	\begin{thebibliography}{24}%
		\makeatletter
		\providecommand \@ifxundefined [1]{%
			\@ifx{#1\undefined}
		}%
		\providecommand \@ifnum [1]{%
			\ifnum #1\expandafter \@firstoftwo
			\else \expandafter \@secondoftwo
			\fi
		}%
		\providecommand \@ifx [1]{%
			\ifx #1\expandafter \@firstoftwo
			\else \expandafter \@secondoftwo
			\fi
		}%
		\providecommand \natexlab [1]{#1}%
		\providecommand \enquote  [1]{``#1''}%
		\providecommand \bibnamefont  [1]{#1}%
		\providecommand \bibfnamefont [1]{#1}%
		\providecommand \citenamefont [1]{#1}%
		\providecommand \href@noop [0]{\@secondoftwo}%
		\providecommand \href [0]{\begingroup \@sanitize@url \@href}%
		\providecommand \@href[1]{\@@startlink{#1}\@@href}%
		\providecommand \@@href[1]{\endgroup#1\@@endlink}%
		\providecommand \@sanitize@url [0]{\catcode `\\12\catcode `\$12\catcode
			`\&12\catcode `\#12\catcode `\^12\catcode `\_12\catcode `\%12\relax}%
		\providecommand \@@startlink[1]{}%
		\providecommand \@@endlink[0]{}%
		\providecommand \url  [0]{\begingroup\@sanitize@url \@url }%
		\providecommand \@url [1]{\endgroup\@href {#1}{\urlprefix }}%
		\providecommand \urlprefix  [0]{URL }%
		\providecommand \Eprint [0]{\href }%
		\providecommand \doibase [0]{https://doi.org/}%
		\providecommand \selectlanguage [0]{\@gobble}%
		\providecommand \bibinfo  [0]{\@secondoftwo}%
		\providecommand \bibfield  [0]{\@secondoftwo}%
		\providecommand \translation [1]{[#1]}%
		\providecommand \BibitemOpen [0]{}%
		\providecommand \bibitemStop [0]{}%
		\providecommand \bibitemNoStop [0]{.\EOS\space}%
		\providecommand \EOS [0]{\spacefactor3000\relax}%
		\providecommand \BibitemShut  [1]{\csname bibitem#1\endcsname}%
		\let\auto@bib@innerbib\@empty
		%</preamble>
		\bibitem [{\citenamefont {Arfken}\ and\ \citenamefont {Weber}(1995)}]{Arfken}%
		\BibitemOpen
		\bibfield  {author} {\bibinfo {author} {\bibfnamefont {G.~B.}\ \bibnamefont
				{Arfken}}\ and\ \bibinfo {author} {\bibfnamefont {H.~J.}\ \bibnamefont
				{Weber}},\ }\href@noop {} {\emph {\bibinfo {title} {Mathematical Methods for
					Physicists}}},\ \bibinfo {edition} {4th}\ ed.\ (\bibinfo  {publisher}
		{Academic Press},\ \bibinfo {address} {San Diego, CA},\ \bibinfo {year}
		{1995})\BibitemShut {NoStop}%
		\bibitem [{\citenamefont {Datta}(1995)}]{datta_1995}%
		\BibitemOpen
		\bibfield  {author} {\bibinfo {author} {\bibfnamefont {S.}~\bibnamefont
				{Datta}},\ }\href {https://doi.org/10.1017/CBO9780511805776} {\emph {\bibinfo
				{title} {Electronic Transport in Mesoscopic Systems}}},\ Cambridge Studies in
		Semiconductor Physics and Microelectronic Engineering\ (\bibinfo  {publisher}
		{Cambridge University Press},\ \bibinfo {year} {1995})\BibitemShut {NoStop}%
		\bibitem [{\citenamefont {Aharonov}\ and\ \citenamefont
			{Bohm}(1959)}]{Aharonov-Bohm:cikk}%
		\BibitemOpen
		\bibfield  {author} {\bibinfo {author} {\bibfnamefont {Y.}~\bibnamefont
				{Aharonov}}\ and\ \bibinfo {author} {\bibfnamefont {D.}~\bibnamefont
				{Bohm}},\ }\bibfield  {title} {\bibinfo {title} {Significance of
				electromagnetic potentials in the quantum theory},\ }\href@noop {} {\bibfield
			{journal} {\bibinfo  {journal} {Phys. Rev.}\ }\textbf {\bibinfo {volume}
				{115}},\ \bibinfo {pages} {485} (\bibinfo {year} {1959})}\BibitemShut
		{NoStop}%
		\bibitem [{\citenamefont {Berry}(1980)}]{Berry_1980}%
		\BibitemOpen
		\bibfield  {author} {\bibinfo {author} {\bibfnamefont {M.~V.}\ \bibnamefont
				{Berry}},\ }\bibfield  {title} {\bibinfo {title} {Exact {Aharonov-Bohm}
				wavefunction obtained by applying {D}irac{'}s magnetic phase factor},\
		}\href@noop {} {\bibfield  {journal} {\bibinfo  {journal} {European Journal
					of Physics}\ }\textbf {\bibinfo {volume} {1}},\ \bibinfo {pages} {240}
			(\bibinfo {year} {1980})}\BibitemShut {NoStop}%
		\bibitem [{\citenamefont {Berry}\ \emph {et~al.}(1980)\citenamefont {Berry},
			\citenamefont {Chambers}, \citenamefont {Large}, \citenamefont {Upstill},\
			and\ \citenamefont {Walmsley}}]{Berry_Chambers_1980}%
		\BibitemOpen
		\bibfield  {author} {\bibinfo {author} {\bibfnamefont {M.~V.}\ \bibnamefont
				{Berry}}, \bibinfo {author} {\bibfnamefont {R.~G.}\ \bibnamefont {Chambers}},
			\bibinfo {author} {\bibfnamefont {M.~D.}\ \bibnamefont {Large}}, \bibinfo
			{author} {\bibfnamefont {C.}~\bibnamefont {Upstill}},\ and\ \bibinfo {author}
			{\bibfnamefont {J.~C.}\ \bibnamefont {Walmsley}},\ }\bibfield  {title}
		{\bibinfo {title} {Wavefront dislocations in the {Aharonov-Bohm} effect and
				its water wave analogue},\ }\href@noop {} {\bibfield  {journal} {\bibinfo
				{journal} {European Journal of Physics}\ }\textbf {\bibinfo {volume} {1}},\
			\bibinfo {pages} {154} (\bibinfo {year} {1980})}\BibitemShut {NoStop}%
		\bibitem [{\citenamefont {Gradshteyn}\ and\ \citenamefont
			{Ryzhik}(1994)}]{Grads:book}%
		\BibitemOpen
		\bibfield  {author} {\bibinfo {author} {\bibfnamefont {I.~S.}\ \bibnamefont
				{Gradshteyn}}\ and\ \bibinfo {author} {\bibfnamefont {I.~M.}\ \bibnamefont
				{Ryzhik}},\ }\href@noop {} {\emph {\bibinfo {title} {Table of Integrals,
					Series, and Products}}},\ \bibinfo {edition} {5th}\ ed.\ (\bibinfo
		{publisher} {Academic Press},\ \bibinfo {address} {London, UK},\ \bibinfo
		{year} {1994})\BibitemShut {NoStop}%
		\bibitem [{\citenamefont {Novoselov}\ \emph {et~al.}(2005)\citenamefont
			{Novoselov}, \citenamefont {Geim}, \citenamefont {Morozov}, \citenamefont
			{Jiang}, \citenamefont {Katsnelson}, \citenamefont {Grigorieva},
			\citenamefont {Dubonos},\ and\ \citenamefont {Firsov}}]{Novoselov2005}%
		\BibitemOpen
		\bibfield  {author} {\bibinfo {author} {\bibfnamefont {K.~S.}\ \bibnamefont
				{Novoselov}}, \bibinfo {author} {\bibfnamefont {A.~K.}\ \bibnamefont {Geim}},
			\bibinfo {author} {\bibfnamefont {S.~V.}\ \bibnamefont {Morozov}}, \bibinfo
			{author} {\bibfnamefont {D.}~\bibnamefont {Jiang}}, \bibinfo {author}
			{\bibfnamefont {M.~I.}\ \bibnamefont {Katsnelson}}, \bibinfo {author}
			{\bibfnamefont {I.~V.}\ \bibnamefont {Grigorieva}}, \bibinfo {author}
			{\bibfnamefont {S.~V.}\ \bibnamefont {Dubonos}},\ and\ \bibinfo {author}
			{\bibfnamefont {A.~A.}\ \bibnamefont {Firsov}},\ }\bibfield  {title}
		{\bibinfo {title} {Two-dimensional gas of massless dirac fermions in
				graphene},\ }\href@noop {} {\bibfield  {journal} {\bibinfo  {journal}
				{Nature}\ }\textbf {\bibinfo {volume} {438}},\ \bibinfo {pages} {197}
			(\bibinfo {year} {2005})}\BibitemShut {NoStop}%
		\bibitem [{\citenamefont {Zhang}\ \emph {et~al.}(2005)\citenamefont {Zhang},
			\citenamefont {Tan}, \citenamefont {Stormer},\ and\ \citenamefont
			{Kim}}]{Zhang2005}%
		\BibitemOpen
		\bibfield  {author} {\bibinfo {author} {\bibfnamefont {Y.}~\bibnamefont
				{Zhang}}, \bibinfo {author} {\bibfnamefont {Y.-W.}\ \bibnamefont {Tan}},
			\bibinfo {author} {\bibfnamefont {H.~L.}\ \bibnamefont {Stormer}},\ and\
			\bibinfo {author} {\bibfnamefont {P.}~\bibnamefont {Kim}},\ }\bibfield
		{title} {\bibinfo {title} {Experimental observation of the quantum hall
				effect and berry's phase in graphene},\ }\href@noop {} {\bibfield  {journal}
			{\bibinfo  {journal} {Nature}\ }\textbf {\bibinfo {volume} {438}},\ \bibinfo
			{pages} {201} (\bibinfo {year} {2005})}\BibitemShut {NoStop}%
		\bibitem [{\citenamefont {DiVincenzo}\ and\ \citenamefont
			{Mele}(1984)}]{DiVincenzo_Mele_PRB_29_1685:ref}%
		\BibitemOpen
		\bibfield  {author} {\bibinfo {author} {\bibfnamefont {D.~P.}\ \bibnamefont
				{DiVincenzo}}\ and\ \bibinfo {author} {\bibfnamefont {E.~J.}\ \bibnamefont
				{Mele}},\ }\bibfield  {title} {\bibinfo {title} {Self-consistent
				effective-mass theory for intralayer screening in graphite intercalation
				compounds},\ }\href {https://doi.org/10.1103/PhysRevB.29.1685} {\bibfield
			{journal} {\bibinfo  {journal} {Phys. Rev. B}\ }\textbf {\bibinfo {volume}
				{29}},\ \bibinfo {pages} {1685} (\bibinfo {year} {1984})}\BibitemShut
		{NoStop}%
		\bibitem [{\citenamefont {Castro~Neto}\ \emph {et~al.}(2009)\citenamefont
			{Castro~Neto}, \citenamefont {Guinea}, \citenamefont {Peres}, \citenamefont
			{Novoselov},\ and\ \citenamefont {Geim}}]{RevModPhys.81.109}%
		\BibitemOpen
		\bibfield  {author} {\bibinfo {author} {\bibfnamefont {A.~H.}\ \bibnamefont
				{Castro~Neto}}, \bibinfo {author} {\bibfnamefont {F.}~\bibnamefont {Guinea}},
			\bibinfo {author} {\bibfnamefont {N.~M.~R.}\ \bibnamefont {Peres}}, \bibinfo
			{author} {\bibfnamefont {K.~S.}\ \bibnamefont {Novoselov}},\ and\ \bibinfo
			{author} {\bibfnamefont {A.~K.}\ \bibnamefont {Geim}},\ }\bibfield  {title}
		{\bibinfo {title} {The electronic properties of graphene},\ }\href
		{https://doi.org/10.1103/RevModPhys.81.109} {\bibfield  {journal} {\bibinfo
				{journal} {Rev. Mod. Phys.}\ }\textbf {\bibinfo {volume} {81}},\ \bibinfo
			{pages} {109} (\bibinfo {year} {2009})}\BibitemShut {NoStop}%
		\bibitem [{\citenamefont {Alford}\ and\ \citenamefont
			{Wilczek}(1989)}]{Wilczek_PhysRevLett.62.1071}%
		\BibitemOpen
		\bibfield  {author} {\bibinfo {author} {\bibfnamefont {M.~G.}\ \bibnamefont
				{Alford}}\ and\ \bibinfo {author} {\bibfnamefont {F.}~\bibnamefont
				{Wilczek}},\ }\bibfield  {title} {\bibinfo {title} {{Aharonov-Bohm}
				interaction of cosmic strings with matter},\ }\href@noop {} {\bibfield
			{journal} {\bibinfo  {journal} {Phys. Rev. Lett.}\ }\textbf {\bibinfo
				{volume} {62}},\ \bibinfo {pages} {1071} (\bibinfo {year}
			{1989})}\BibitemShut {NoStop}%
		\bibitem [{\citenamefont {Gerbert}(1989)}]{Gerbert_PhysRevD.40.1346}%
		\BibitemOpen
		\bibfield  {author} {\bibinfo {author} {\bibfnamefont {P.~d.~S.}\
				\bibnamefont {Gerbert}},\ }\bibfield  {title} {\bibinfo {title} {Fermions in
				an {Aharonov-Bohm} field and cosmic strings},\ }\href@noop {} {\bibfield
			{journal} {\bibinfo  {journal} {Phys. Rev. D}\ }\textbf {\bibinfo {volume}
				{40}},\ \bibinfo {pages} {1346} (\bibinfo {year} {1989})}\BibitemShut
		{NoStop}%
		\bibitem [{\citenamefont {Hagen}(1990)}]{Hagen_PhysRevLett.64.503}%
		\BibitemOpen
		\bibfield  {author} {\bibinfo {author} {\bibfnamefont {C.~R.}\ \bibnamefont
				{Hagen}},\ }\bibfield  {title} {\bibinfo {title} {{Aharonov-Bohm} scattering
				of particles with spin},\ }\href@noop {} {\ \textbf {\bibinfo {volume}
				{64}},\ \bibinfo {pages} {503} (\bibinfo {year} {1990})}\BibitemShut
		{NoStop}%
		\bibitem [{\citenamefont {Hagen}\ and\ \citenamefont
			{Ramaswamy}(1990)}]{Hagen_PhysRevD.42.3524}%
		\BibitemOpen
		\bibfield  {author} {\bibinfo {author} {\bibfnamefont {C.~R.}\ \bibnamefont
				{Hagen}}\ and\ \bibinfo {author} {\bibfnamefont {S.}~\bibnamefont
				{Ramaswamy}},\ }\bibfield  {title} {\bibinfo {title} {{Aharonov-Bohm}
				scattering of massive spin-one particles},\ }\href@noop {} {\bibfield
			{journal} {\bibinfo  {journal} {Phys. Rev. D}\ }\textbf {\bibinfo {volume}
				{42}},\ \bibinfo {pages} {3524} (\bibinfo {year} {1990})}\BibitemShut
		{NoStop}%
		\bibitem [{\citenamefont {Novoselov}\ \emph {et~al.}(2006)\citenamefont
			{Novoselov}, \citenamefont {McCann}, \citenamefont {Morozov}, \citenamefont
			{Fal'ko}, \citenamefont {Katsnelson}, \citenamefont {Zeitler}, \citenamefont
			{Jiang}, \citenamefont {Schedin},\ and\ \citenamefont
			{Geim}}]{Novoselov_Hall:ref}%
		\BibitemOpen
		\bibfield  {author} {\bibinfo {author} {\bibfnamefont {K.}~\bibnamefont
				{Novoselov}}, \bibinfo {author} {\bibfnamefont {E.}~\bibnamefont {McCann}},
			\bibinfo {author} {\bibfnamefont {S.}~\bibnamefont {Morozov}}, \bibinfo
			{author} {\bibfnamefont {V.}~\bibnamefont {Fal'ko}}, \bibinfo {author}
			{\bibfnamefont {M.}~\bibnamefont {Katsnelson}}, \bibinfo {author}
			{\bibfnamefont {U.}~\bibnamefont {Zeitler}}, \bibinfo {author} {\bibfnamefont
				{D.}~\bibnamefont {Jiang}}, \bibinfo {author} {\bibfnamefont
				{F.}~\bibnamefont {Schedin}},\ and\ \bibinfo {author} {\bibfnamefont
				{A.}~\bibnamefont {Geim}},\ }\bibfield  {title} {\bibinfo {title}
			{{Unconventional quantum Hall effect and Berry's phase of 2 pi in bilayer
					graphene}},\ }\href@noop {} {\bibfield  {journal} {\bibinfo  {journal}
				{Nature Phys.}\ }\textbf {\bibinfo {volume} {{2}}},\ \bibinfo {pages} {177}
			(\bibinfo {year} {{2006}})}\BibitemShut {NoStop}%
		\bibitem [{\citenamefont {McCann}\ and\ \citenamefont
			{Fal'ko}(2006)}]{mccann:086805}%
		\BibitemOpen
		\bibfield  {author} {\bibinfo {author} {\bibfnamefont {E.}~\bibnamefont
				{McCann}}\ and\ \bibinfo {author} {\bibfnamefont {V.~I.}\ \bibnamefont
				{Fal'ko}},\ }\bibfield  {title} {\bibinfo {title} {Landau-level degeneracy
				and quantum hall effect in a graphite bilayer},\ }\href@noop {} {\bibfield
			{journal} {\bibinfo  {journal} {Phys. Rev. Lett.}\ }\textbf {\bibinfo
				{volume} {96}},\ \bibinfo {eid} {086805} (\bibinfo {year}
			{2006})}\BibitemShut {NoStop}%
		\bibitem [{\citenamefont {Rashba}(1960)}]{Rashba_cikk_1960}%
		\BibitemOpen
		\bibfield  {author} {\bibinfo {author} {\bibfnamefont {E.}~\bibnamefont
				{Rashba}},\ }\bibfield  {title} {\bibinfo {title} {Properties of
				semiconductors with an extremum loop. i. cyclotron and combinational
				resonance in a magnetic field perpendicular to the plane of the loop},\
		}\href@noop {} {\bibfield  {journal} {\bibinfo  {journal} {Sov. Phys.-Solid
					State}\ }\textbf {\bibinfo {volume} {2}},\ \bibinfo {pages} {1109} (\bibinfo
			{year} {1960})}\BibitemShut {NoStop}%
		\bibitem [{\citenamefont {Bychkov}\ and\ \citenamefont
			{Rashba}(1984)}]{Yu_A_Bychkov_1984}%
		\BibitemOpen
		\bibfield  {author} {\bibinfo {author} {\bibfnamefont {Y.~A.}\ \bibnamefont
				{Bychkov}}\ and\ \bibinfo {author} {\bibfnamefont {E.~I.}\ \bibnamefont
				{Rashba}},\ }\bibfield  {title} {\bibinfo {title} {Oscillatory effects and
				the magnetic susceptibility of carriers in inversion layers},\ }\href@noop {}
		{\bibfield  {journal} {\bibinfo  {journal} {Journal of Physics C: Solid State
					Physics}\ }\textbf {\bibinfo {volume} {17}},\ \bibinfo {pages} {6039}
			(\bibinfo {year} {1984})}\BibitemShut {NoStop}%
		\bibitem [{\citenamefont {\ifmmode \check{Z}\else
				\v{Z}\fi{}uti\ifmmode~\acute{c}\else \'{c}\fi{}}\ \emph
			{et~al.}(2004)\citenamefont {\ifmmode \check{Z}\else
				\v{Z}\fi{}uti\ifmmode~\acute{c}\else \'{c}\fi{}}, \citenamefont {Fabian},\
			and\ \citenamefont {Das~Sarma}}]{Fabian_RevModPhys.76.323}%
		\BibitemOpen
		\bibfield  {author} {\bibinfo {author} {\bibfnamefont {I.}~\bibnamefont
				{\ifmmode \check{Z}\else \v{Z}\fi{}uti\ifmmode~\acute{c}\else \'{c}\fi{}}},
			\bibinfo {author} {\bibfnamefont {J.}~\bibnamefont {Fabian}},\ and\ \bibinfo
			{author} {\bibfnamefont {S.}~\bibnamefont {Das~Sarma}},\ }\bibfield  {title}
		{\bibinfo {title} {Spintronics: Fundamentals and applications},\ }\href@noop
		{} {\bibfield  {journal} {\bibinfo  {journal} {Rev. Mod. Phys.}\ }\textbf
			{\bibinfo {volume} {76}},\ \bibinfo {pages} {323} (\bibinfo {year}
			{2004})}\BibitemShut {NoStop}%
		\bibitem [{\citenamefont {Winkler}(2003)}]{Winkler:684956}%
		\BibitemOpen
		\bibfield  {author} {\bibinfo {author} {\bibfnamefont {R.}~\bibnamefont
				{Winkler}},\ }\href@noop {} {\emph {\bibinfo {title} {{Spin-orbit coupling
						effects in two-dimensional electron and hole systems}}}},\ Springer Tracts in
		Modern Physics\ (\bibinfo  {publisher} {Springer},\ \bibinfo {address}
		{Berlin},\ \bibinfo {year} {2003})\BibitemShut {NoStop}%
		\bibitem [{\citenamefont {Urban}\ \emph {et~al.}(2011)\citenamefont {Urban},
			\citenamefont {Bercioux}, \citenamefont {Wimmer},\ and\ \citenamefont
			{H\"ausler}}]{PhysRevB.84.115136}%
		\BibitemOpen
		\bibfield  {author} {\bibinfo {author} {\bibfnamefont {D.~F.}\ \bibnamefont
				{Urban}}, \bibinfo {author} {\bibfnamefont {D.}~\bibnamefont {Bercioux}},
			\bibinfo {author} {\bibfnamefont {M.}~\bibnamefont {Wimmer}},\ and\ \bibinfo
			{author} {\bibfnamefont {W.}~\bibnamefont {H\"ausler}},\ }\bibfield  {title}
		{\bibinfo {title} {Barrier transmission of dirac-like pseudospin-one
				particles},\ }\href@noop {} {\bibfield  {journal} {\bibinfo  {journal} {Phys.
					Rev. B}\ }\textbf {\bibinfo {volume} {84}},\ \bibinfo {pages} {115136}
			(\bibinfo {year} {2011})}\BibitemShut {NoStop}%
		\bibitem [{\citenamefont {Shen}\ \emph {et~al.}(2010)\citenamefont {Shen},
			\citenamefont {Shao}, \citenamefont {Wang},\ and\ \citenamefont
			{Xing}}]{PhysRevB.81.041410}%
		\BibitemOpen
		\bibfield  {author} {\bibinfo {author} {\bibfnamefont {R.}~\bibnamefont
				{Shen}}, \bibinfo {author} {\bibfnamefont {L.~B.}\ \bibnamefont {Shao}},
			\bibinfo {author} {\bibfnamefont {B.}~\bibnamefont {Wang}},\ and\ \bibinfo
			{author} {\bibfnamefont {D.~Y.}\ \bibnamefont {Xing}},\ }\bibfield  {title}
		{\bibinfo {title} {Single dirac cone with a flat band touching on
				line-centered-square optical lattices},\ }\href@noop {} {\bibfield  {journal}
			{\bibinfo  {journal} {Phys. Rev. B}\ }\textbf {\bibinfo {volume} {81}},\
			\bibinfo {pages} {041410} (\bibinfo {year} {2010})}\BibitemShut {NoStop}%
		\bibitem [{\citenamefont {Bercioux}\ \emph {et~al.}(2009)\citenamefont
			{Bercioux}, \citenamefont {Urban}, \citenamefont {Grabert},\ and\
			\citenamefont {H\"ausler}}]{PhysRevA.80.063603}%
		\BibitemOpen
		\bibfield  {author} {\bibinfo {author} {\bibfnamefont {D.}~\bibnamefont
				{Bercioux}}, \bibinfo {author} {\bibfnamefont {D.~F.}\ \bibnamefont {Urban}},
			\bibinfo {author} {\bibfnamefont {H.}~\bibnamefont {Grabert}},\ and\ \bibinfo
			{author} {\bibfnamefont {W.}~\bibnamefont {H\"ausler}},\ }\bibfield  {title}
		{\bibinfo {title} {Massless dirac-weyl fermions in a ${\mathcal{t}}_{3}$
				optical lattice},\ }\href@noop {} {\bibfield  {journal} {\bibinfo  {journal}
				{Phys. Rev. A}\ }\textbf {\bibinfo {volume} {80}},\ \bibinfo {pages} {063603}
			(\bibinfo {year} {2009})}\BibitemShut {NoStop}%
		\bibitem [{\citenamefont {D\'ora}\ \emph {et~al.}(2011)\citenamefont {D\'ora},
			\citenamefont {Kailasvuori},\ and\ \citenamefont
			{Moessner}}]{PhysRevB.84.195422}%
		\BibitemOpen
		\bibfield  {author} {\bibinfo {author} {\bibfnamefont {B.}~\bibnamefont
				{D\'ora}}, \bibinfo {author} {\bibfnamefont {J.}~\bibnamefont
				{Kailasvuori}},\ and\ \bibinfo {author} {\bibfnamefont {R.}~\bibnamefont
				{Moessner}},\ }\bibfield  {title} {\bibinfo {title} {Lattice generalization
				of the dirac equation to general spin and the role of the flat band},\
		}\href@noop {} {\bibfield  {journal} {\bibinfo  {journal} {Phys. Rev. B}\
			}\textbf {\bibinfo {volume} {84}},\ \bibinfo {pages} {195422} (\bibinfo
			{year} {2011})}\BibitemShut {NoStop}%
	\end{thebibliography}%
	
\end{document}
